# Supplementary material for: GRAPHEVAL: Quantifying Reasoning Uncertainty to Assess Trustworthiness in LLMs
Source: arXiv:2607.08017 source file (2026-12-02)
Supplement: Supplementary file 1 [file broad_attack_appendix.tex]

\begin{comment}
\begin{figure}[h]
%\begin{wrapfigure}{r}{0.85\textwidth}
    \centering
    %\includegraphics[width=\linewidth]
    \includegraphics[scale=0.26]{pic/scatter_medqa.pdf} 
    \caption{\textbf{Population Level Medoid Ablation}. 
    \textit{Methodology}: For each question and model, we follow the same ablation strategy detailed in \Cref{fig:broad_ablation_fig}.
    \textit{Results}: Many points lie near $\Delta$Accuracy$=0$ but below $\Delta$Faithfulness$=0$, showing a reduction reasoning fidelity. This is strongest for Phi-4 and Llama 3.1 8B ($r=-0.17$, $p=0.011$ For Llama 3.1 8B; $r=-0.18$, $p=0.010$ for Phi-4), and largely absent for DeepSeek-R1 ($r=-0.01$, $p=0.856$), though the latter still shows mild faithfulness loss for nearly 50\% of questions with near-zero accuracy change.} %while the baselines remain weak.} 
    %\rreva{remove this (already in main paper), put two or three other datasets, like medqa gpqa for sure}
    \label{fig:broad_ablation_fig_appendix}
    %\vspace{-5mm}
\end{figure}
%\end{wrapfigure}
\end{comment}
\begin{figure}[htbp]
    \centering
    
    
    % 2. GSM8K
    \begin{subfigure}{\textwidth}
        \centering
        \includegraphics[width=0.85\linewidth]{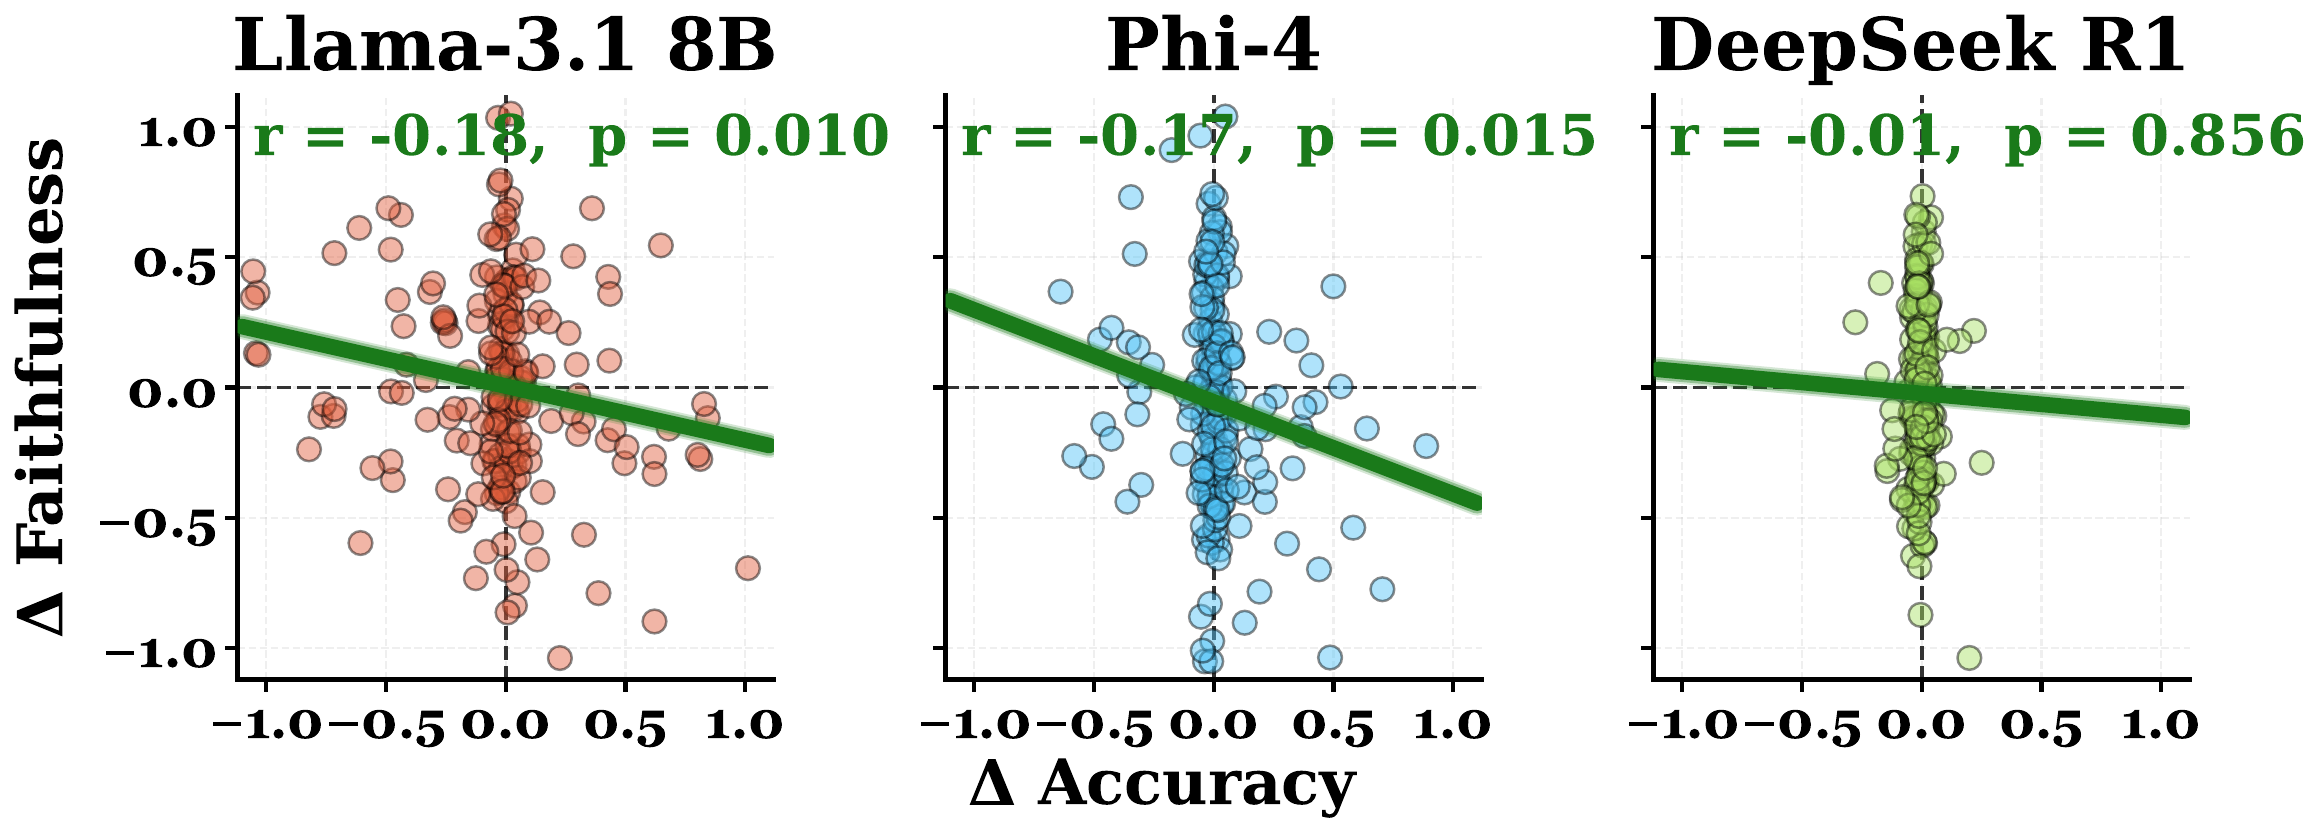}
        \caption{\textbf{GSM8K}}
        \label{fig:scatter_gsm8k}
    \end{subfigure}
    
    \vspace{0.4cm}
    
    % 3. BoolQ
    \begin{subfigure}{\textwidth}
        \centering
        \includegraphics[width=0.85\linewidth]{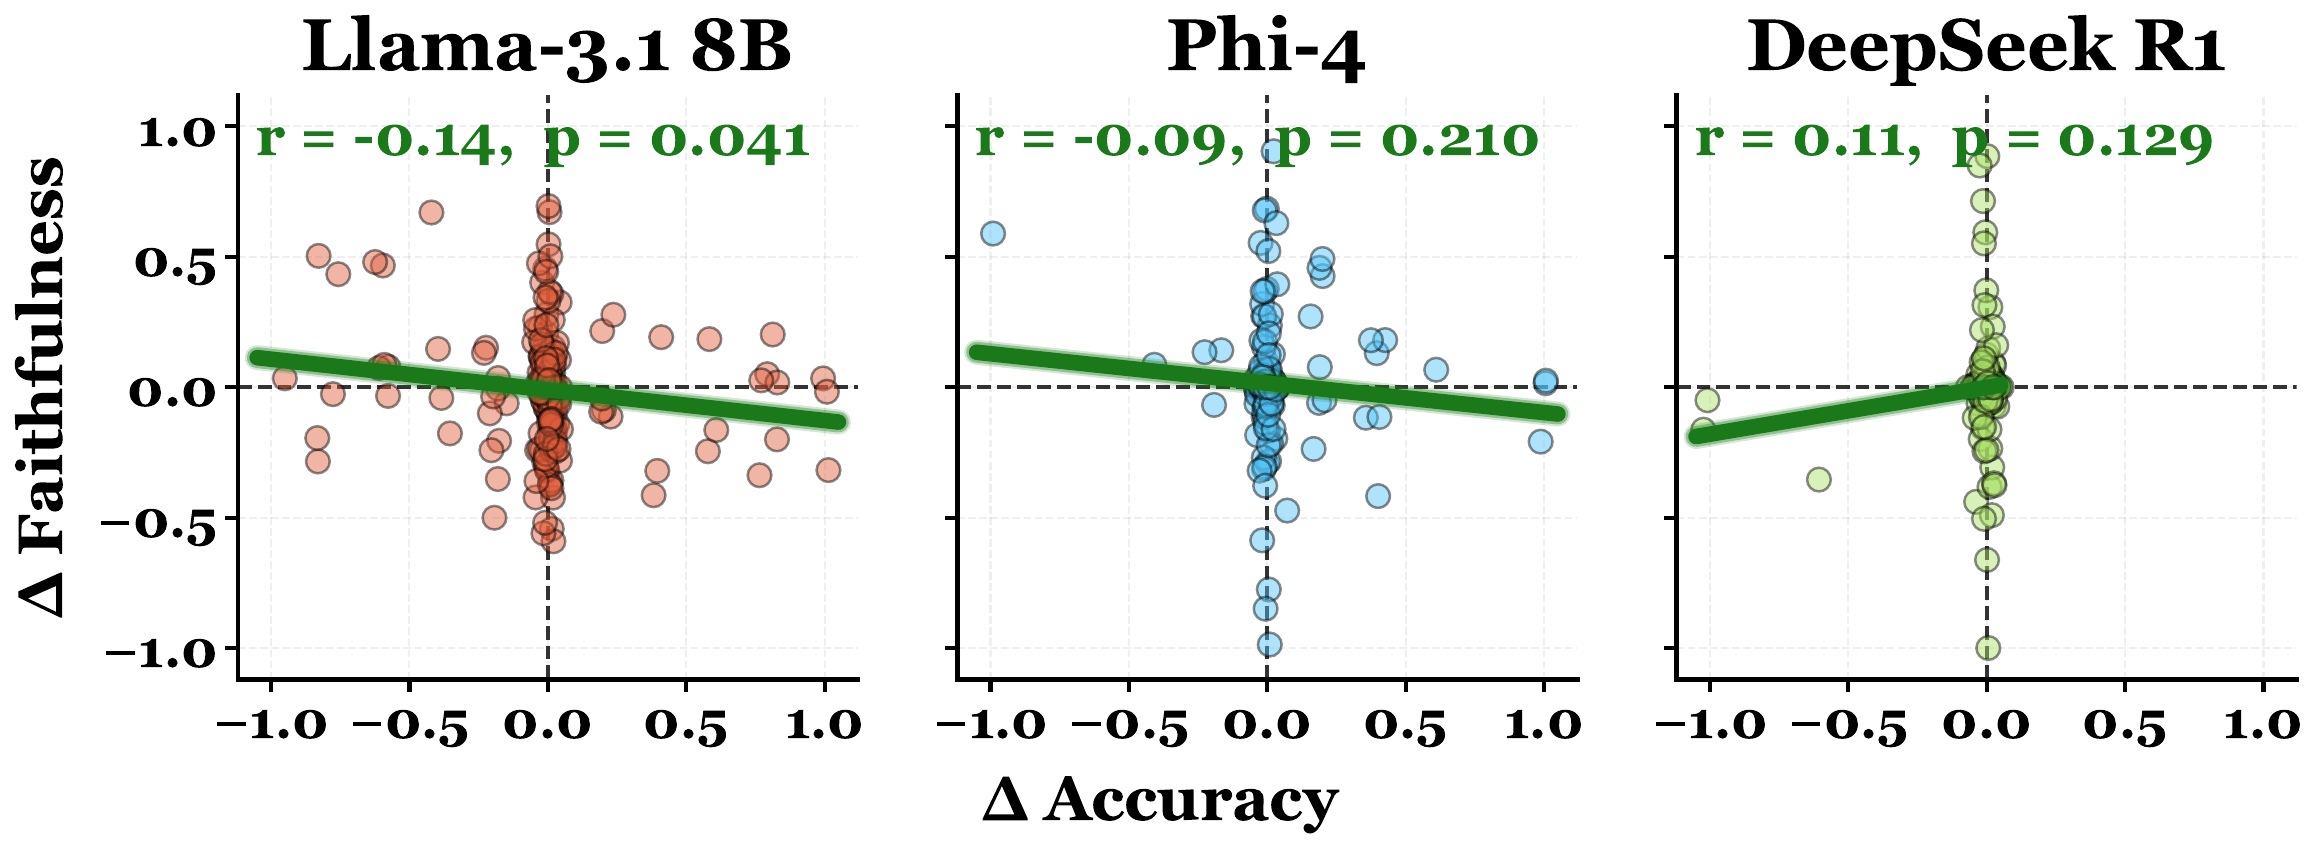}
        \caption{\textbf{BoolQ}}
        \label{fig:scatter_boolq}
    \end{subfigure}
    
    \vspace{0.4cm}

     % 1. MedQA
    \begin{subfigure}{\textwidth}
        \centering
        \includegraphics[width=0.85\linewidth]{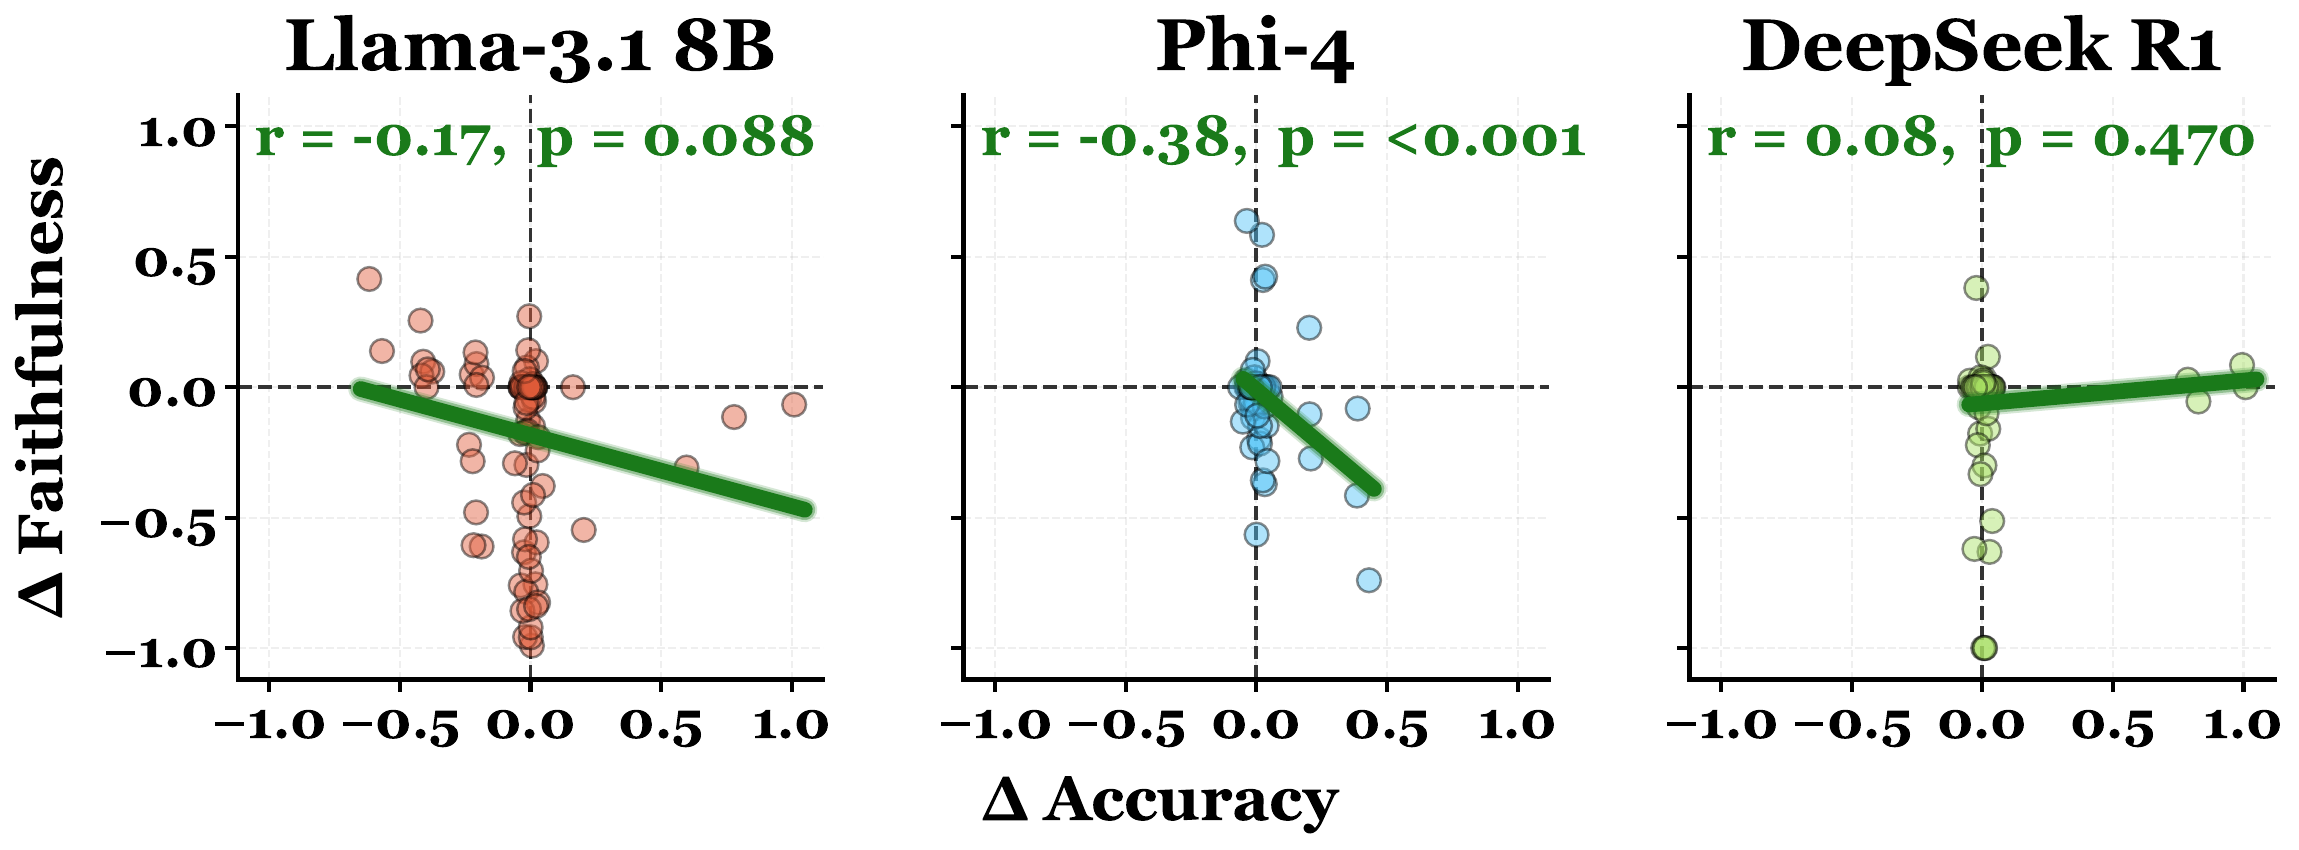}
        \caption{\textbf{MedQA}}
        \label{fig:scatter_medqa}
    \end{subfigure}
    
    \vspace{0.4cm} % Adds a little breathing room between charts
    
    % 4. GPQA
    \begin{subfigure}{\textwidth}
        \centering
        \includegraphics[width=0.85\linewidth]{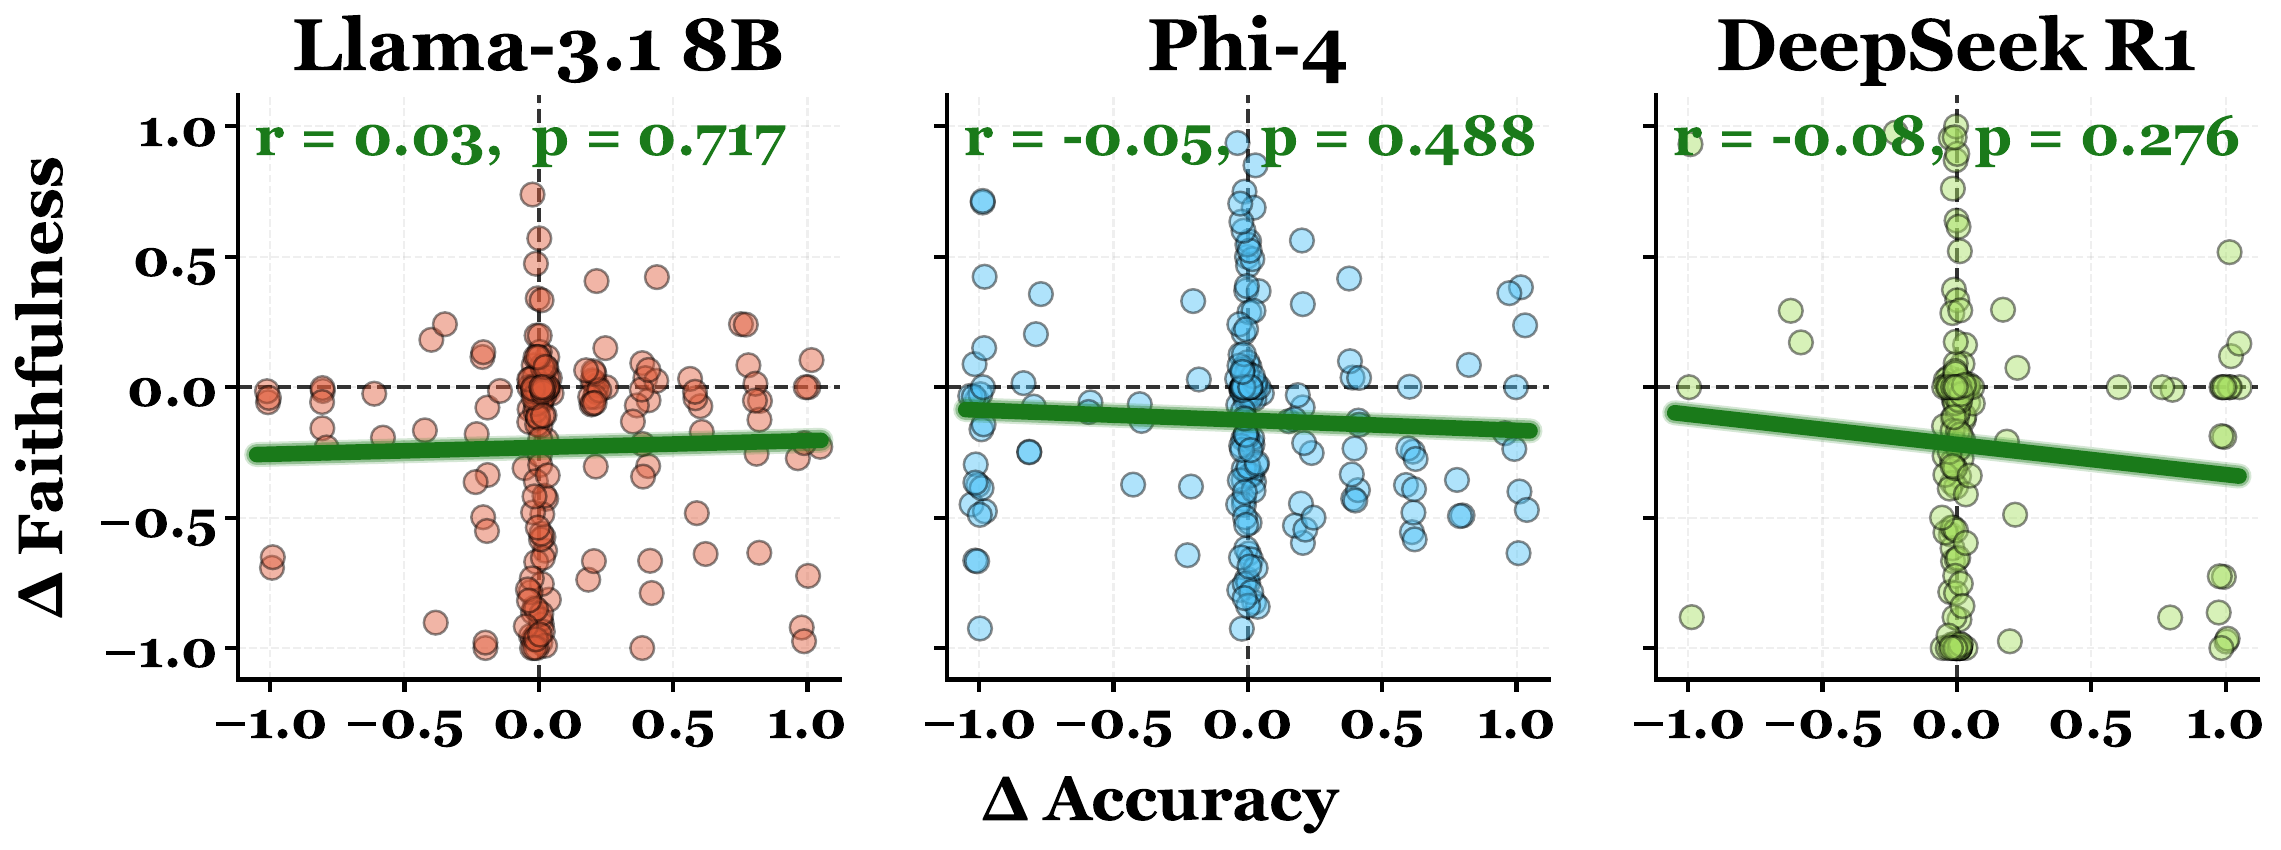}
        \caption{\textbf{GPQA}}
        \label{fig:scatter_gpqa}
    \end{subfigure}

    \caption{\textbf{Population-Level Medoid Ablation Across Diverse Domains}. 
   For smaller GLLMs, accuracy gains couple with faithfulness drops on MedQA and GSM8K (the ``lucky guess'' phenomenon), but weaken on BoolQ and GPQA. Crucially, all datasets show a dense cluster at $\Delta$Accuracy $= 0$ with negative $\Delta$Faithfulness, proving medoid ablation degrades reasoning even when accuracy is preserved.}
    \label{fig:broad_ablation_fig_appendix}
\end{figure}
