# Supplementary material for: GRAPHEVAL: Quantifying Reasoning Uncertainty to Assess Trustworthiness in LLMs
Source: arXiv:2607.08017 source file (2026-12-02)
Supplement: Supplementary file 2 [file krc_src_appendix.tex]

\begin{figure}[t]
%\begin{wrapfigure}{r}{0.85\textwidth}
    \centering
    %\includegraphics[width=\linewidth]
    \includegraphics[scale=0.16]{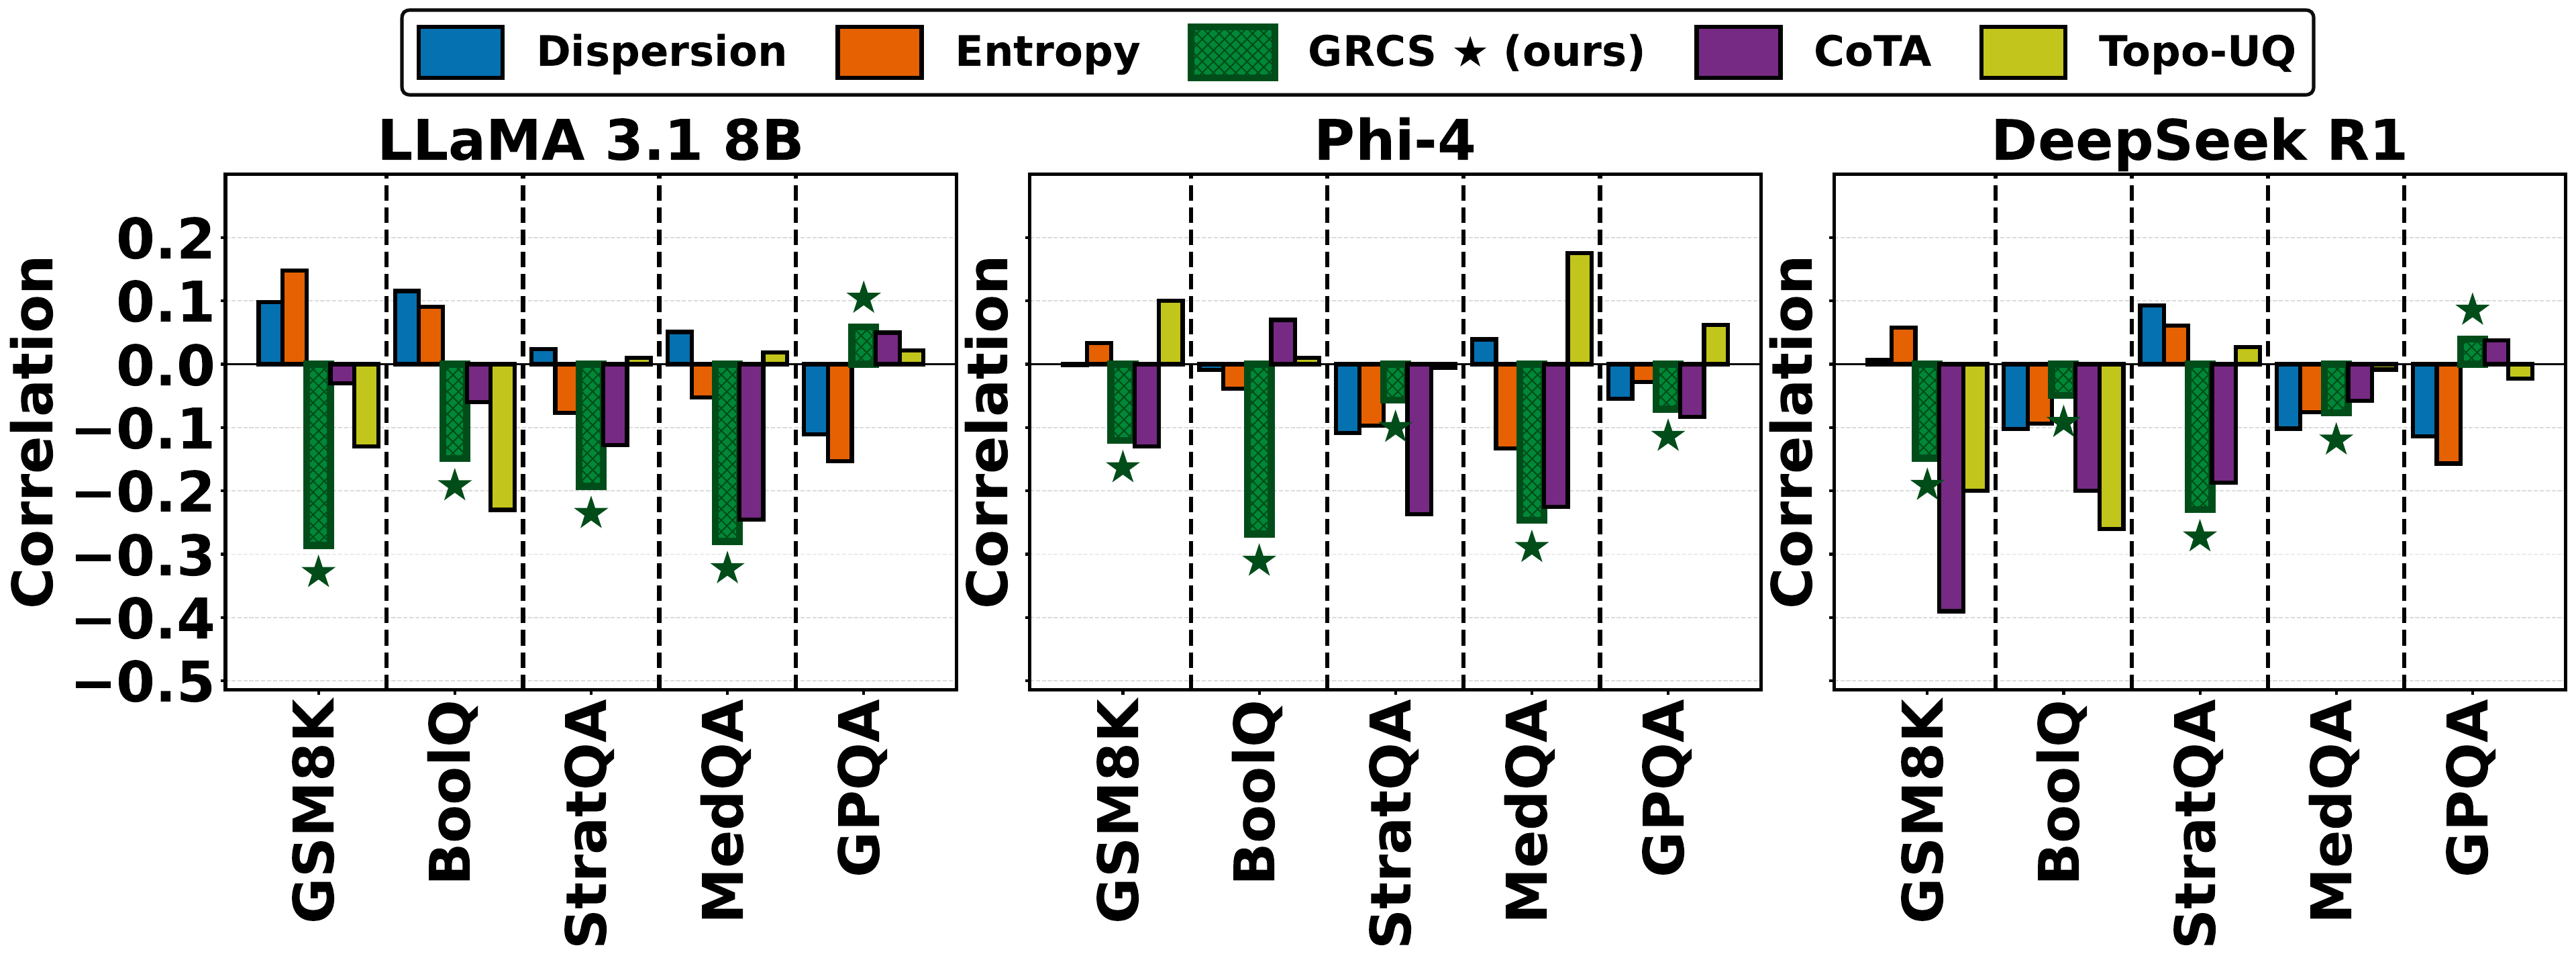} 
    \includegraphics[scale=0.16]{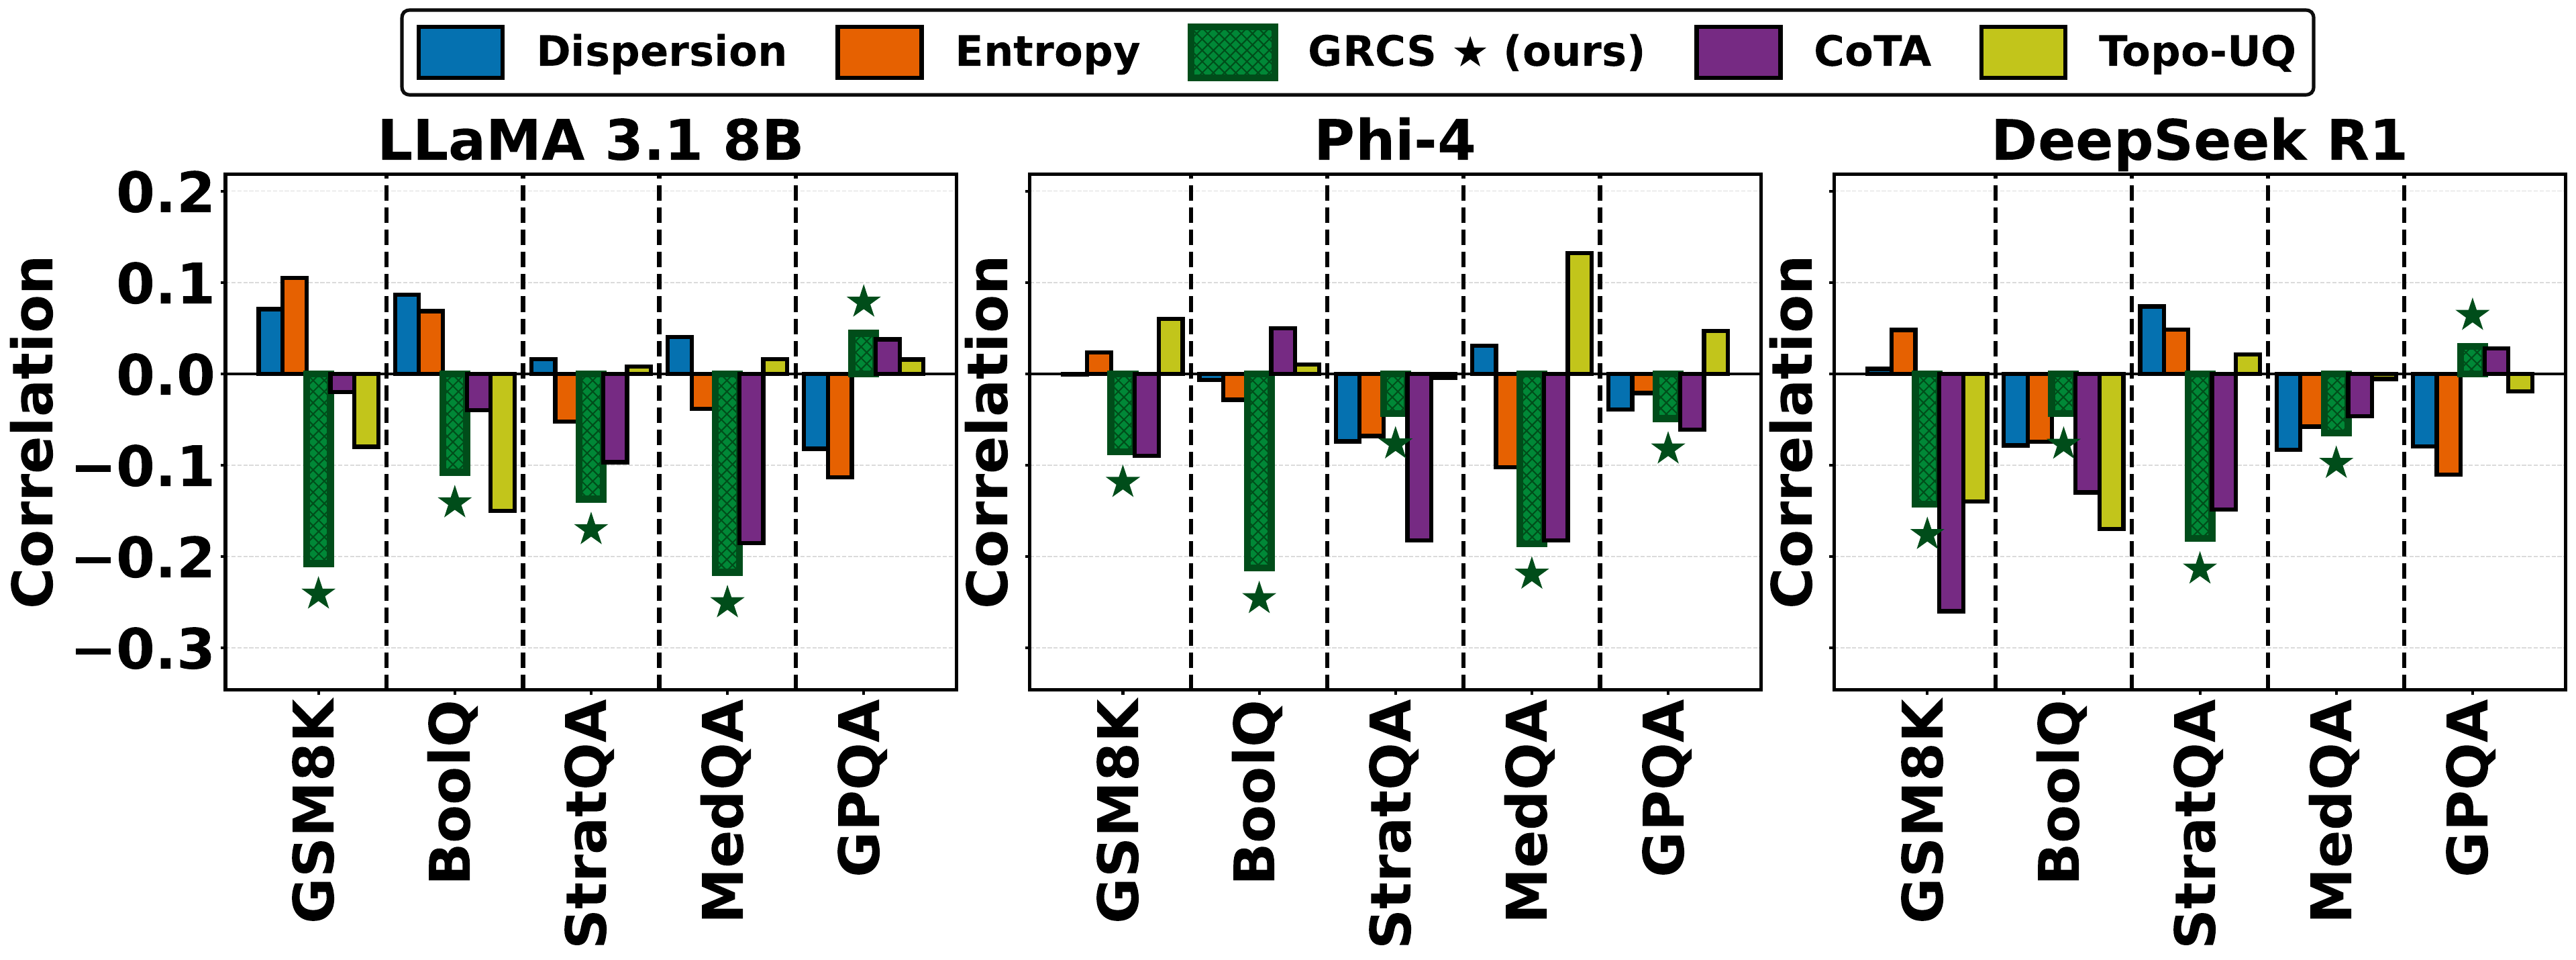} 
    \caption{\textbf{UQ Analysis (SRC \& KRC)}. 
    A stronger negative correlation indicates a better uncertainty metric. GRCS is negatively correlated with faithfulness in $\sim$ 87\% of the (GLLM, dataset) pairs and outperforms all baselines in 7 out of 15 cases. In the hardest setting (GPQA), GRCS, CoTA, and Topo-UQ frequently yield weak or positive correlations.}
    \label{fig:krc_src_appendix}
    %\vspace{-5mm}
\end{figure}
