# Supplementary material for: GRAPHEVAL: Quantifying Reasoning Uncertainty to Assess Trustworthiness in LLMs
Source: arXiv:2607.08017 source file (2026-12-02)
Supplement: Supplementary file 3 [file path_level_appendix.tex]

\begin{figure}
    \centering
    \includegraphics[scale=0.13]{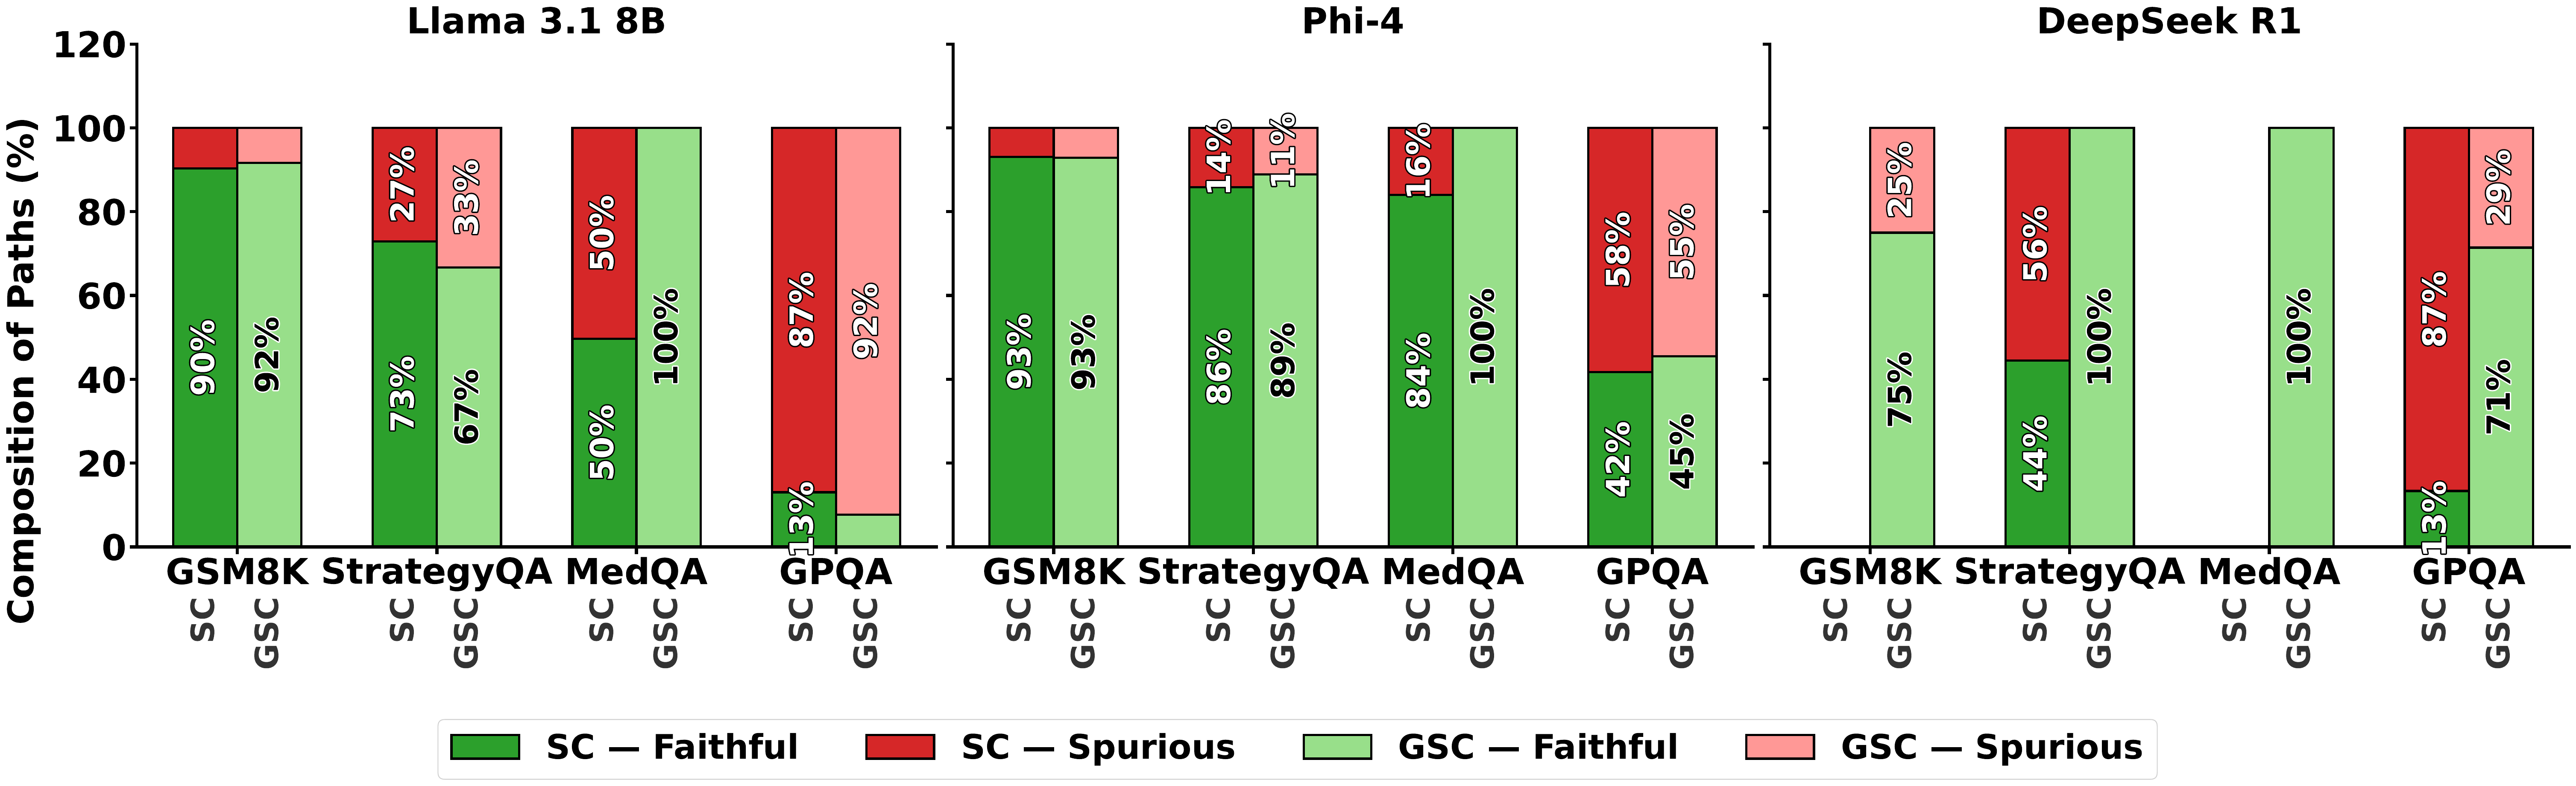} 
    \caption{\textbf{Granular Path-level audit of SC--GSC disagreement cases.} 
   Each stacked bar shows the fraction %share 
    of \textit{faithful} (green) and \textit{spurious} (red) paths within that disagreement cell.
    SC-only paths are often less faithful than GSC-only paths, though the gap varies by model and dataset.  Overall, across 13 comparable disagreement settings (\ie, with both SC-only and GSC-only wins), GSC has a higher faithful share in 7, ties in 1, and is lower in 3.} %\rreva{use same format as paper graph}
    \label{fig:gsc_sc_verification_rate_apppedix}
\end{figure}
