# Supplementary material for: GRAPHEVAL: Quantifying Reasoning Uncertainty to Assess Trustworthiness in LLMs
Source: arXiv:2607.08017 source file (2026-12-02)
Supplement: Supplementary file 4 [file appendix.tex]

\section{Notation Table}

In this section, we provide a comprehensive list of notations and acronyms that we have used in this work as shown in~\Cref{table:notations}.

\vspace{5mm}

\input{tables/notations}


\section{Various Prompts and Mathematical Analysis}
\subsection{Prompts Used in the Pipeline}\label{sec:appendix_prompts}

This appendix reports the prompts used in the final pipeline. For each stage, we first summarize the prompt's role and then provide the exact text.

\subsubsection{GLLM Reasoning Generation Prompt}
This prompt is fed to the GLLM and it's used to generate structured reasoning traces. It instructs the model to produce a concise sequence of reasoning steps (from $n_l = 3$ to $n_h = 6$), where each step is defined as a single \emph{declarative sentence} stating one fact or conclusion. The steps need to be numbered and annotated with their direct \emph{causal dependencies}. At the end of its reasoning, the model needs to output the final answer to the question following a precise, structured format. This format allows the reasoning path to be translated %parsed 
into a graph representation.

\begin{lstlisting}[
  style=promptstyle,
  caption={GLLM Reasoning Generation Prompt},
  label={lst:GLLM_prompt},
  emph={Given,Guidelines,Output,Number,depends_on,If,Do,not,Question,final,answer, declarative, question}
]
You are a careful and logical reasoner.
Given a question, produce a step-by-step reasoning chain that leads to an answer.

Guidelines:
- Output a number of steps that is between 3 and 6, depending on the complexity of the question. Avoid excessive verbosity or unnecessary steps. Be straightforward and concise, but ensure the reasoning is complete and clear.
- Each step is a single declarative sentence stating one fact or conclusion.
- Number each step starting from 0.
- After each step, on the same line, write [depends_on: N, M, ...] listing the indices of ALL prior steps this step directly requires to be derived.
  If the step is a new premise requiring no prior steps, write [depends_on: none].
- Do not include titles, headers, or any extra text.
- Do not use XML tags or hidden-thought markers such as <think>,
  </think>, <reasoning>, or similar.
- Do not repeat the question.
- Do not output lists or bullet points beyond the numbered steps.
- At the end, on its own line, write: \"The final answer is: [answer]\"

Question: {QUESTION}
\end{lstlisting}

\subsubsection{DLLM Atomic Decomposition Prompt}
This prompt is fed to the DLLM to decompose each reasoning step into atomic \emph{Subject--Verb--Object} facts. Crucially, it preserves the original step index and dependency annotations, ensuring that graph granularity is refined without altering the logical structure of the original reasoning trace. The DLLM is also given a decomposition example, following the \emph{Few Shots Prompting} technique \cite{brown2020languagemodels}.

\begin{lstlisting}[
  style=promptstyle,
  caption={DLLM Atomic Decomposition Prompt},
  label={lst:DLLM_prompt},
  emph={Rules,atomic,fact,step,depends_on,DO,NOT,CHANGE,DEPENDENCIES,Replace,Output,ONLY,Example,input,output,Now}
]
You are a precise sentence decomposer.

You will receive a numbered reasoning chain with [depends_on: ...] annotations.
Decompose each step into atomic facts while preserving its step index and
dependency annotation.

Rules:
- Each atomic fact must express one independent fact in subject-verb-object form.
- Every fact from step N must keep [step: N, depends_on: ...] exactly as given.
- DO NOT CHANGE OR INFER DEPENDENCIES.
- Prefix each fact with ###.
- Replace pronouns with the original subject.
- Do not repeat, rephrase, or invent facts.
- Output ONLY annotated atomic facts.

Example input:
0. A standard matchbox has internal dimensions of approximately 1.5 x 0.75 x 0.5 inches. [depends_on: none]
1. A nickel has a diameter of 0.835 inches and a thickness of 0.077 inches. [depends_on: none]
2. The nickel fits within the matchbox dimensions. [depends_on: 0, 1]

Example output:
### A standard matchbox has an internal length of approximately 1.5 inches. [step: 0, depends_on: none]
### A standard matchbox has an internal width of approximately 0.75 inches. [step: 0, depends_on: none]
### A standard matchbox has an internal height of approximately 0.5 inches. [step: 0, depends_on: none]
### A nickel has a diameter of 0.835 inches. [step: 1, depends_on: none]
### A nickel has a thickness of 0.077 inches. [step: 1, depends_on: none]
### The nickel fits within the matchbox dimensions. [step: 2, depends_on: 0, 1]

Now decompose this reasoning chain:

{REASONING_PATH}
\end{lstlisting}

\subsubsection{GLLM Adversarial Attack Prompt}\label{sec:adv_prompt_appendix}
This prompt is used in the adversarial medoid ablation experiment to test whether the GSC-selected medoid is a load-bearing reasoning path. It requires the GLLM to answer the same question while explicitly avoiding the medoid’s logic, allowing us to measure whether accuracy and reasoning faithfulness deteriorate when that path is removed. As in the standard generation stage, the output must follow the same structured reasoning format.

\begin{lstlisting}[
  style=promptstyle,
  caption={GLLM Adversarial Attack Prompt},
  label={lst:ADV_prompt},
  emph={CRITICAL,CONSTRAINT,STRICTLY,FORBIDDEN,COMPLETELY,ALTERNATIVE,Guidelines,depends_on,Do,not,Question,final,answer,reasoning, alternative}
]
You are a careful and logical reasoner.
Given a question, produce a step-by-step reasoning chain that leads to an answer.

CRITICAL CONSTRAINT: You are strictly forbidden from using the following
reasoning path or logical steps:
<forbidden_reasoning>
{MEDOID_TEXT}
</forbidden_reasoning>

You must find a completely alternative, valid way to reason through the
problem from scratch. Do not copy the logic of the forbidden reasoning.

Guidelines:
- Output between 3 and 6 steps.
- Each step is a single declarative sentence.
- Number each step starting from 0.
- After each step, write [depends_on: N, M, ...] listing the prior steps.
  If the step relies on no prior steps, write [depends_on: none].
- Do not include headers, bullet points, or extra text.
- Do not use XML tags or hidden-thought markers such as <think>,
  </think>, <reasoning>, or similar.
- Clearly display the reasoning in the final response.
- At the end, on its own line, write:
  "The final answer is: [answer]"

Question: {QUESTION}
\end{lstlisting}

\subsection{GED Formulation}\label{sec:ged_def_appendix}
The Graph Edit Distance (GED), theorized by \cite{sanfeliu1983distance} and further expanded by \cite{riesen2009approximate}, measures the similarity between two graphs, $G_i$ (\emph{source graph}) and $G_j$ (\emph{target graph}), by computing the minimum cost of modifications required to transform $G_i$ into $G_j$. The transformation is achieved through \emph{edit operations}, that are typically user defined and encompass the insertion, deletion, and substitution of both nodes and edges. Let an edit path be a sequence of edit operations $(e_1, \dots, e_k)$ that completely transforms $G_i$ into $G_j$. GED is defined as the minimum total cost among all possible edit sequences:$$GED(G_i, G_j) = \min_{(e_1, \dots, e_k) \in \Upsilon(G_i, G_j)} \sum_{x=1}^k c(e_x)$$where $\Upsilon(G_i, G_j)$ denotes the set of all valid edit sequences transforming $G_i$ into $G_j$, and $c(e_x)$ represents the non-negative cost associated with a specific edit operation $e_x$.
The exact computation of GED relies on combinatorial search algorithms (such as $A^*$ search \cite{hart1968formal}), it is computationally prohibitive when we need to study deep graphs, because its complexity scales exponentially with the number of nodes. %Let $m = \max(|V_i|, |V_j|)$ denote the maximum node count between the two evaluated graphs, %specifically 
%this approach has complexity of $\mathcal{O}(|V_j|^{|V_i|})$ (where $|V_i|$ and $|V_j|$ are the node counts of $G_i$ and $G_j$, respectively). 
Let $m = \max(|V_i|, |V_j|)$ denote the maximum node count between the two evaluated graphs. The exact computation of GED %relies 
has thus a time complexity of $\mathcal{O}(|V_j|^{|V_i|})$, which scales exponentially as $\mathcal{O}(m^m)$ in the worst case.
To overcome this NP-hard bottleneck, our framework leverages the Hungarian algorithm, introduced by \cite{korsah2007dynamic}, which approximates this task to an optimal bipartite matching problem. Refer to \Cref{sec:ss_ged_appendix} for the detailed explanation of our approach.

\subsection{Detailed SS-GED Definition}\label{sec:ss_ged_appendix}
For each question $q$, we obtain a set of $N$ reasoning graphs $\{G_1,\dots,G_N\}$ and compute pairwise distances between all graph pairs. Let $G_i=(V_i,E_i)$ and $G_j=(V_j,E_j)$ denote two DAGs derived from sampled reasoning chains. Our goal is to quantify both \emph{structural divergence} and \emph{semantic disagreement} between them.

\smallskip
\noindent {\bf Node and Edge Matching.}
We first construct a bipartite cost matrix between graph elements and solve the assignment problem with the Hungarian algorithm \cite{korsah2007dynamic}. Rather than exploring all possible edit sequences, we decouple the matching process into independent assignments for nodes and edges. For any two matched elements (either nodes or edges) $a$ and $b$, the substitution cost is defined by cosine distance:
\[
c_{\text{sub}}(a,b)=1-\frac{\langle \mathbf{z}_a,\mathbf{z}_b\rangle}{\|\mathbf{z}_a\|\|\mathbf{z}_b\|},
\]
where $\mathbf{z}_a$ and $\mathbf{z}_b$ are the corresponding embedding vectors. Insertions and deletions are assigned unit cost. This yields a raw semantic-aware edit cost, denoted $C_{\text{edit}}(G_i,G_j)$, that is computed as the sum of the optimal substitution costs (the summation over matched pairs) and the unit insertion/deletion costs for any unmatched elements (the absolute difference in graph cardinalities):
\[
Cost_{V} = \sum_{(u,v) \in P^*_{V}} c_{\text{sub}}(u, v) + \big| |V_i| - |V_j| \big|
\]
\[
Cost_{E} = \sum_{(e_i,e_j) \in P^*_{E}} c_{\text{sub}}(e_i, e_j) + \big| |E_i| - |E_j| \big|
\]
\[
C_{\text{edit}}(G_i,G_j) = Cost_{V} + Cost_{E}
\]

In the worst case, our approach, leveraging the bipartite mathcing, operates with a time complexity of $\mathcal{O}(m^3)$, where $m = \max(|V_i|, |V_j|)$. This reduction from exponential to cubic complexity makes the evaluation of deep graphs computationally feasible ($\cf$, \Cref{fig:complexity_comparison}).
\input{pic/complexitygraph}

\smallskip
\noindent {\bf Fair Normalization.}
Because reasoning graphs can differ substantially in length, we normalize the raw edit cost by the average graph size rather than by a single graph alone:
\[
\mathrm{nGED}(G_i,G_j)=
\frac{C_{\text{edit}}(G_i,G_j)}
{\frac{|V_i|+|V_j|}{2}}.
\]
This makes the comparison scale depend symmetrically on both graphs and avoids over-penalizing pairs in which one chain is much longer than the other.

\smallskip
\noindent {\bf Terminal Semantic Agreement.}
Topology alone is insufficient, since two reasoning chains may share similar structure but reach different conclusions. To capture this, we compute a terminal semantic score from the terminal nodes of each DAG. Let
\[
T_i=\{v\in V_i:\mathrm{outdeg}(v)=0\},
\qquad
T_j=\{v\in V_j:\mathrm{outdeg}(v)=0\},
\]
be the terminal-node sets. Their aggregate embeddings are
\[
\bar{\mathbf{t}}_i=\frac{1}{|T_i|}\sum_{v\in T_i}\mathbf{z}_v,
\qquad
\bar{\mathbf{t}}_j=\frac{1}{|T_j|}\sum_{v\in T_j}\mathbf{z}_v.
\]
We then define terminal semantic similarity as
\[
S_{\text{term}}(G_i,G_j)=
\frac{\langle \bar{\mathbf{t}}_i,\bar{\mathbf{t}}_j\rangle}
{\|\bar{\mathbf{t}}_i\|\|\bar{\mathbf{t}}_j\|}.
\]

\smallskip
\noindent {\bf Semantic-Structural Blending.}
We convert normalized edit distance into a bounded structural similarity through an RBF \cite{scholkopf2002learning} transform:
\[
S_{\text{struct}}(G_i,G_j)=\exp\!\bigl(-\gamma\,\mathrm{nGED}(G_i,G_j)^2\bigr),
\]
where $\gamma>0$ controls how sharply similarity decays as structural divergence increases. The final SS-GED similarity is then defined as
\[
S_{\text{SS-GED}}(G_i,G_j)
=
\beta\,S_{\text{term}}(G_i,G_j)
+
(1-\beta)\,S_{\text{struct}}(G_i,G_j),
\]
where $\beta\in[0,1]$ controls the trade-off between semantic outcome agreement and internal structural consistency. The final distance is
\[
d_{\text{SS-GED}}(G_i,G_j)=1-S_{\text{SS-GED}}(G_i,G_j).
\]

\smallskip
\noindent {\bf Hyperparameter Choice.}
We use a single global configuration across all experiments, fixing $\beta=0.4$ and $\gamma=5.0$. The choice $\beta=0.4$ places slightly greater emphasis on structural consistency while still allowing conclusion-level semantic agreement to affect the score. This weighting is specifically designed to counteract the "lucky guess" phenomenon, where fragmented or hallucinated paths accidentally converge on a correct final label. The choice $\gamma=5.0$ yields a moderately sharp RBF decay, so that small structural differences are not over-amplified while clearly distinct graphs remain well separated. These values are kept fixed across all models and datasets, with no per-task hyperparameter tuning.

\subsection{Mathematical Justification for the RBF Kernel in SS-GED}\label{sec_rbf_appendix}
\input{pic/rbf_appendix}
In our SS-GED computation, we map the normalized Graph Edit Distance ($nGED$) to a bounded similarity measure $[0, 1]$ using a Radial Basis Function (RBF) kernel, also known as a Gaussian kernel \cite{scholkopf2002learning}:$$S_{struct}(G_i, G_j) = \exp(-\gamma \cdot nGED(G_i, G_j)^2)$$ where $G_i$ and $G_j$ represent a pair of DAGs. The choice of an RBF kernel over a linear decay ($\eg$, $1 - nGED$) is motivated by the nature of LLMs' reasoning paths. In high-dimensional reasoning spaces, structural variation may be \emph{non-linear} rather than well captured by simple Euclidean scaling \cite{meila2024manifold}. As result, we choose to use an RBF transform to convert nGED to a bounded similarity measure by smoothly separating more distant graphs.
As shown in \Cref{fig:rbf_fig_appendix}, a linear decay model treats every unit of edit distance with equal weight. Under such a regime, a reasoning path that is $50\%$ structurally different would still retain $0.5$ similarity. However, in complex tasks like clinical ($\eg$ MedQA) or expert reasoning ($\eg$, GPQA), a $50\%$ divergence in causal nodes typically indicates a significant departure from the established logical manifold, that is not accurately captured by linear representations. By contrast, the RBF kernel with $\gamma = 5.0$ establishes a \emph{High-Fidelity Plateau} at low $nGED$ values ($<0.1$), where its relatively flat Gaussian curve ensures that minor decomposition artifacts do not fragment the structural consensus. This offer an advantage compare to linear decay, which over-penalizes very close structural variations. As nGED increases, the RBF kernel enters an \emph{Accelerated Penalty Zone}, where squared exponent drives similarity toward zero far more aggressively than a linear model. In this region, \bem{the RBF kernel more clearly separates significantly different reasoning paths}. The parameter $\gamma$ sets the width of the Gaussian kernel. The choice of $\gamma = 5.0$ is a middle ground between two extremes. A low $\gamma$ (e.g., $0.1$) is too permissive, failing to penalize major structural differences and allowing incompatible paths to score highly. In contrast, a high $\gamma$ (e.g., $20.0$) is too sensitive, where small, non-semantic differences push similarity toward zero, fragmenting consensus..

\subsection{Detailed GSC Definition}\label{sec_gsc_detailed_appendix}
\smallskip
\noindent {\bf Detailed GSC Scoring.}
Given the set of $N=20$ reasoning graphs for a query, we first compute the full pairwise SS-GED distance matrix and convert it to a similarity matrix,
\[
S(G_i,G_j)=1-d_{\text{SS-GED}}(G_i,G_j).
\]

\smallskip
\noindent {\bf Structural Centrality.}
We define the global centrality of a graph $G_i$ as its total similarity to the rest of the pool:
\[
C(G_i)=\sum_{j\neq i} S(G_i,G_j).
\]
Graphs with high $C(G_i)$ lie near the center of the reasoning manifold and therefore represent dominant semantic-structural patterns shared across samples.

\smallskip
\noindent {\bf Node-Level Support.}
Centrality alone is not sufficient, since a graph may be globally typical while still containing isolated hallucinated steps. To capture local support, we compute a node-level consensus score. For each node $v\in G_i$, let $\mathbf{z}_v$ be its embedding. We define
\[
c(v)=\frac{1}{N-1}\sum_{j\neq i}\mathbf{1}\!\left[\max_{u\in G_j}\cos(\mathbf{z}_v,\mathbf{z}_u)\ge \tau\right],
\]
where $\tau=0.9$ is the semantic support threshold and $\mathbf{1}[\cdot]$ is the indicator function. Thus, $c(v)$ measures the fraction of other graphs containing at least one highly semantically related node.

\smallskip
\noindent {\bf Path Consensus.}
We aggregate node support into a graph-level consensus score,
\[
P(G_i)=\frac{\sum_{v\in V_i} w(v)\,c(v)}{\sum_{v\in V_i} w(v)},
\]
where
\[
w(v)=
\begin{cases}
2.0, & \text{if } \mathrm{outdeg}(v)=0,\\
1.0, & \text{otherwise.}
\end{cases}
\]
Terminal nodes are upweighted because they encode the final conclusion of the reasoning chain. An unsupported terminal claim can make the entire CoT incorrect even if earlier intermediate steps are locally plausible. In contrast, unsupported intermediate nodes may be less critical if later steps do not rely on them directly.

\smallskip
\noindent {\bf Final Medoid Selection.}
The final GSC score combines normalized global centrality with local path consensus:
\[
\mathrm{Score}(G_i)=
\alpha\,\frac{C(G_i)}{\max_k C(G_k)}+(1-\alpha)\,P(G_i).
\]
We then select
\[
G^\star=\arg\max_{G_i}\mathrm{Score}(G_i),
\]
as the final \bem{medoid} path, and return the final answer associated with $G^\star$, considered as the GSC's final prediction. In all experiments, we fix $\alpha=0.8$, prioritizing structural centrality while allowing path consensus to filter out centrally located but weakly supported traces. We found the framework to be qualitatively stable across nearby values of $\alpha$. 

\subsection{Detailed Adversarial Medoid Ablation Protocol
%\dpal{Needs correction}
}\label{sec:abl_appendix}
For each question \(q\), let $x_q$ denote the original %input 
prompt presented to each GLLM (as defined in \Cref{lst:GLLM_prompt}). %and let \(z_q^\star\) denote the medoid CoT selected by GSC. 
Let $z_q$ denote a generic CoT
sampled from the GLLM given $x_q$, and let $z_q^\star$ denote the GSC-selected medoid CoT.
We design a prompt that directly suppresses the medoid's logic. 
Let $\delta_{\mathrm{ablate}}(z_q^\star)$ denote an adversarial perturbation instruction constructed from $z_q^\star$. It is a natural-language instruction that (i) presents $z_q^\star$ in full, (ii) explicitly forbids the model from reusing any of its reasoning steps or conclusions, and (iii) instructs the model to produce a completely alternative CoT from scratch. We can then formalize the adversarial prompt as:
$$
x_q' = x_q \cup \delta_{\mathrm{ablate}}(z_q^\star)
$$
where $\cup$ denotes prompt concatenation. Refer to \Cref{lst:ADV_prompt} for the detailed adversarial prompt used in our experiments.
By construction, $x_q'$ steers the model away from $z_q^\star$. As result, it restricts 
the reasoning space from which the alternative CoTs are sampled.
We instantiate this attack under two complementary protocols.

\begin{comment}
We construct an adversarially perturbed prompt
\[
x_q' = x_q \oplus \delta_{\mathrm{ablate}}(z_q^\star),
\]
where \(\delta_{\mathrm{ablate}}\) injects the full medoid reasoning into the prompt as explicitly \emph{forbidden reasoning} and instructs the model to produce a completely alternative step-by-step chain from scratch. In all cases, the model is required to output a 3--6 step CoT with explicit dependency annotations and a final answer line. The exact prompt template is reported in Appendix \ref{sec:adv_prompt_appendix}. Our implementation uses this same perturbation in both attack settings.
\rreva{update this too}
\smallskip
\fixme{RR: ABLATION METHODOLOGY UPDATE!!!!! Look at main paper}
\noindent {\bf Targeted Ablation.}
The targeted setting operates on the subset of questions where GSC is correct and SC is incorrect. For each such question, we generate a single adversarial alternative \(z_q^{\mathrm{adv}}\) at deterministic temperature \(T=0.0\), and evaluate whether removing the medoid logic causes degradation in answer correctness, reasoning faithfulness, or both. This isolates the causal importance of the selected medoid precisely in the regime where GSC provides a decoding advantage over SC.
\end{comment}

\smallskip
\noindent {\bf Broad Population-Level Medoid Ablation.}
The broad setting applies the same attack to all datasets questions. For each question \(q\), we sample \(N\) adversarial alternative CoTs:
\[
\mathcal{Z}_q^{\mathrm{adv}}=\{z_{q,1}^{\mathrm{adv}},\dots,z_{q,N}^{\mathrm{adv}}\}
\]
at temperature \(T\) (in practice, we use $N=20$ and $T=7$, to capture the GLLM's reasoning diversity, as we did within the original pipeline), and aggregate them into stable per-question estimates. For MedQA, we follow the main evaluation protocol and use a fixed random subsample of 100 questions (seed 42). This broad protocol estimates the average causal effect of medoid ablation at the dataset level rather than only on the narrow disagreement subset.

\smallskip
\noindent {\bf Targeted Medoid Ablation.}
The targeted setting operates on the subset of questions where GSC is correct and SC is incorrect. For each such question, we generate $N$ adversarial alternative CoTs at temperature $T$ (in practice, we resort to $N = 20$ and $T=7$ to follow the main paper experiments). This isolates the causal importance of the selected medoid precisely in the regime where GSC provides a decoding advantage over SC. Due to page limit, this experiment is deferred to Appendix \ref{sec_target_appendix}.

In both protocols, alternative paths are evaluated along three dimensions: \textit{ablated accuracy}, \textit{ablated faithfulness}, and \textit{medoid distance}.

\smallskip
\noindent {\bf Ablated %Alternative 
Accuracy.}
Given a gold answer $y_q$, the accuracy of an adversarial alternative CoT $z_{q,k}^{\mathrm{adv}}$ is
\[
A_{q,k}^{\mathrm{adv}}=\mathbf{1}\!\left[\hat{y}(z_{q,k}^{\mathrm{adv}})=y_q\right],
\]
where $\hat{y}(\cdot)$ extracts the final answer from the generated CoT and $\mathbf{1}$ is the indicator function. In both protocols,
we average across the $N$ alternatives:
\[
A_q^{\mathrm{adv}}=\frac{1}{N}\sum_{k=1}^{N} A_{q,k}^{\mathrm{adv}}.
\]
For comparison, the baseline medoid accuracy is
\[
A_q^{\star}=\mathbf{1}\!\left[\hat{y}(z_q^\star)=y_q\right],
\]
and the accuracy drop under ablation is
\[
\Delta A_q = A_q^{\mathrm{adv}} - A_q^\star.
\]

\smallskip
\noindent {\bf Ablated %Alternative 
Faithfulness.}
Faithfulness is evaluated with the same Early Answering procedure used in the main 
evaluation protocol. Let $f_{q,k,1},\dots,f_{q,k,n_{q,k}}$ be the atomic facts obtained 
by decomposing $z_{q,k}^{\mathrm{adv}}$. For each prefix $f_{q,k,1:i}$, we reprompt the 
model to answer using only that partial context. If the correct answer is already recoverable 
from an early prefix, the chain is treated as less faithful. Formally,
\[
m_{q,k,i}=
\mathbf{1}\!\left[\hat{y}\!\bigl(\mathrm{EA}(q,f_{q,k,1:i})\bigr)=y_q\right],
\]
and the adversarial faithfulness of $z_{q,k}^{\mathrm{adv}}$ is
\[
F_{q,k}^{\mathrm{adv}}
=
1-\frac{1}{n_{q,k}}\sum_{i=1}^{n_{q,k}} m_{q,k,i}.
\]
In both protocols, we average across the $N$ alternatives:
\[
F_q^{\mathrm{adv}}=\frac{1}{N}\sum_{k=1}^{N}F_{q,k}^{\mathrm{adv}}.
\]
We compare against the baseline medoid faithfulness $F_q^\star$, computed via the same 
Early Answering procedure applied to $z_q^\star$, and define
\[
\Delta F_q = F_q^{\mathrm{adv}} - F_q^\star.
\]
%The scripts 
%We implement this by decomposing each adversarial CoT into facts, querying the model on incrementally expanding prefixes, and computing faithfulness as one minus the fraction of prefixes that already recover the correct answer.

\smallskip
\noindent {\bf Medoid Distance.}
To quantify how far each adversarial alternative CoT $z_{q,k}^{\mathrm{adv}}$ is from the medoid $z_q^\star$, we compute 
normalized sequence dissimilarity:
\[
D_{q,k}^{\mathrm{med}}
=
1-\mathrm{sim}\!\left(z_q^\star, z_{q,k}^{\mathrm{adv}}\right),
\]
where $\mathrm{sim}(\cdot,\cdot)\in[0,1]$ is a normalized sequence similarity measure 
between two CoT texts. In practice, it is the longest-common-subsequence 
ratio on lowercased text. We deliberately use a lightweight, model-free surface measure 
here rather than SS-GED, to perform an unbiased, graph-independent evaluation.
Thus $D_{q,k}^{\mathrm{med}}=0$ indicates identical texts, while 
larger values reflect greater deviation from the forbidden medoid logic. We report the 
per-question average
\[
D_q^{\mathrm{med}}=\frac{1}{N}\sum_{k=1}^{N}D_{q,k}^{\mathrm{med}},
\]
which serves as an empirical check that $x_q'$ successfully steers GLLMs' reasoning away 
from $z_q^\star$.
%This quantity is used as a proxy for how successfully the attack forces the model away from the original medoid trajectory.

\section{Auxiliary Experimental Results}

\subsection{Evaluation on Long-Horizon Reasoning}
\label{sec:long_horizon_reasoning}

To test our pipeline on a much longer, multi-hop reasoning mathematical dataset, we evaluated on AIME-2026 \cite{dekoninck2026beyond}. We specifically chose this benchmark because, unlike GPQA which spans diverse and highly distinct scientific domains, AIME focuses exclusively on advanced mathematical reasoning. This provides a domain-consistent yet highly cognitively demanding environment, making it an ideal testbed to observe how well uncertainty metrics scale to deeper, multi-step reasoning traces without being confounded by cross-domain variance.

In \Cref{tab:aime_evaluation} we  compare the Pearson Correlation Coefficient (PCC) between Faithfulness and GRCS (ours), CoTA, Topo-UQ, Dispersion, and Entropy. As detailed in our paper, a stronger negative correlation indicates a better uncertainty metric (\Cref{sec:exp_setup}).

\input{tables/aime_arxiv}

\bem{We observe that GRCS provides a better uncertainty metric when evaluating AIME-2026 in two out of three GLLMs, and outperforms CoTA/Topo-UQ in all possible cases.}

\subsection{Scalability to Longer Reasoning Traces}
\label{sec:scalability_extended_cots}

To test the scalability of our pipeline, in \Cref{tab:scalability_ged} where we set the number of reasoning steps to 10--20 (i.e., more than 3x the number of steps we set in the main paper). We observe an increase in volume of the atomic facts. On average, we observe a 2x--3x increase in graph sizes. On the GPQA dataset, for example, DeepSeek goes from $\approx 30$ to $\approx 80$ fact nodes per DAG. For LLama 3.1 8B, the median fact count increases from $\approx 30$ to roughly $\approx 50$, and the maximum outlier range expands significantly, growing from $\approx 600$ to nearly $\approx 1,000$ facts. 

However, the $\pname$ pipeline remains stable. Given that the pipeline complexity is $O(N^2 \cdot m^3)$ (where $m$ is the node count), larger graphs increase computation time as expected. However, our key finding regarding the robustness question raised by the reviewer is that the evaluation remains tractable without correctness violation, as the pipeline gets fully executed without issues. The graph alignment uses the Hungarian algorithm (complexity: $O(m^3)$, where $m = \max(|V_i|, |V_j|)$ and $V_i, V_j$ denote the node sets of graphs $G_i$ and $G_j$, respectively.), which operates on bipartite graphs of arbitrary size and scales to larger DAGs containing hundreds of nodes. 

We validate this stability by comparing the SS-GED for the elicited CoT having 10--20 steps. In Table~\ref{tab:scalability_ged}, we report the average GED and SS-GED for Baseline (i.e., 3--6 reasoning steps per CoT) and Extended (i.e., 10--20 reasoning steps per CoT) runs. While GED increased proportionally with graph size by roughly 2x to 3x across our benchmarks (this behavior is expected, with GED being a raw distance measure, applied on bigger graphs), \bem{the normalized SS-GED remained remarkably consistent. This cancels out length bias between the CoTs.}

\input{tables/longer_traces}

\subsection{Validation via Counterfactual Editing}
\label{sec:counterfactual_editing}

To rigorously isolate the causal impact of individual reasoning steps and validate our faithfulness metric through an independent intervention beyond Early Answering, we introduce a counterfactual editing protocol. We intervene \cite{pearl2009causality,halpern2001causes} on each intermediate step (i.e., excluding the terminal conclusion) of the reasoning path by prompting Mistral-Large 2512 to generate a counterfactual (CF) for that step, while keeping all other steps fixed. We perturbed one step per iteration, and rotated the perturbation across all intermediate steps. This follows the view of counterfactual reasoning formalized by Pearl et al., where causal relevance is assessed by modifying one variable at a time and observing its effect on the outcome \cite{pearl2009causality,halpern2001causes}.

Prior to the full evaluation, we validated the quality of the generated counterfactuals by having one of the authors manually assess 50 randomly sampled counterfactual steps (seed 42) on whether they were plausible but factually distinct from the original step. We then evaluated the same subset using an ``LLM-as-judge'' (Claude 3.6 Sonnet), achieving a Cohen's Kappa of 0.81 with the human evaluation, proving the reliability of the counterfactuals generation.

A step is counted as faithful if altering it changes the final answer (the model accounted for it in its decision making) and unfaithful if the answer is unchanged (the model did not account for it during its decision making). The per-question CF faithfulness score is the fraction of intermediate steps that are faithful. These scores are then correlated with GRCS using the same 1,000-bootstrap PCC procedure as Early Answering (EA), defined in the main paper. Table~\ref{tab:counterfactual_editing} shows the PCC for Early Answering (PCC-EA), for Counterfactual Editing (PCC-CF), and the difference $\Delta(\text{CF} - \text{EA})$ for all GLLMs, across GPQA, MedQA and StrategyQA datasets.

\input{tables/counterfactuals_pearl}

\subsection{Ablation Study on DLLMs}\label{sec:appendix_dllms_ablation}

\input{tables/dllms_ablation_1}
\vspace{3mm}

To evaluate the robustness of the factual decomposition step and ensure our framework is not overly reliant on a single DLLM, we conducted an ablation study using multiple different DLLMs. We compared our primary DLLM (GPT-4o, \Cref{sec:methodology}) with two open-weight, frontier-class LLMs (Mistral-Large-2512 and GPT-OSS-120b) and one commercial frontier-class LLM (Google Gemini 3 Flash). To evaluate the correctness of the decomposition, one of the authors manually evaluated 50 randomly sampled reasoning graphs (seed 42, used to ensure reproducibility) across GPQA, MedQA, and StrategyQA on three criteria: Atomicity (ability of the DLLM to isolate independent claims), Absence of Hallucinations, and Dependency Validity (accurate preservation and mapping of causal topological edges). We then evaluated this same subset using an ``LLM-as-judge'' (Claude 3.6 Sonnet, \cite{gu2026llmjudge}) which achieved a Cohen's Kappa \cite{cohen1960kappa} of 0.82 with the human evaluation (we used a different LLM than the DLLMs under study to avoid self-evaluation biases). We then extended the automated evaluation to 1,500 randomly sampled reasoning graphs across GPQA, MedQA, and StrategyQA (seed 42, used to ensure reproducibility). With 1,500 samples, the reported percentages are statistically stable across random seeds: by the normal approximation to sample proportions, i.e., the de Moivre--Laplace/Central Limit Theorem, the worst-case standard error is minimal. Because the goal is to assess decomposition quality rather than dataset-level task performance, we aggregate results across datasets. For each CoT and its corresponding reasoning graph, we evaluate the atomic facts produced by the DLLM against the original CoT and report the percentage of graph-CoT pairs satisfying each criterion, averaged over the 1,500 graphs from the three datasets (Table~\ref{tab:dllm_quality}). We observe that the pipeline is robust and sufficiently decomposer-agnostic. Absence of Hallucinations is consistently $> 95\%$ across evaluated DLLMs. Atomicity is consistently more than 88\%. This confirms that the evaluated DLLMs are suitable to break reasoning traces into atomic, independent facts. The Dependency Validity scores are lower because occasionally, DLLMs tend to skip transitive logical edges in complex answers.

To assess if our methodology is overly sensitive to the choice of the DLLM, we also executed an Inter-DLLM agreement study, computing the average fact nodes per CoT, and average edges per CoT on GPQA, MedQA and StrategyQA (Table~\ref{tab:dllm_agreement}).

\input{tables/dllms_ablation_2}
\vspace{3mm}

We observe that the average number of facts per CoT and the average number of edges per fact remain consistent with the characteristics of the datasets (GPQA, which is the hardest, requires more facts per CoT on average, followed by MedQA and StrategyQA) and are comparable across the different DLLMs.

Furthermore, fixing the GLLM to Llama-3.1 8B, we report the Pearson Correlation Coefficient (PCC) between the final GRCS score assigned using the baseline GPT-4o DLLM (the DLLM used in the main paper) and the GRCS scores assigned by the three additional DLLMs (Table~\ref{tab:dllm_pcc}):

\input{tables/dllms_ablation_3}
\vspace{3mm}

These high correlations entail that the pipeline is stable across different DLLMs. The lowest agreement occurs for GPT-OSS-120B on StrategyQA (PCC = 0.57) and reflects that StrategyQA is the most challenging dataset for atomic decomposition. Its open-domain commonsense questions rely on informal reasoning that is harder to decompose into clean Subject-Verb-Object atomic facts compared to MedQA and GPQA, which are more structured. MedQA consistently yields the highest correlations (up to 0.94), likely because clinical reasoning follows a highly structured format (e.g., symptoms, diagnosis, treatment) that systematically maps onto atomic Subject-Verb-Object facts with clear causal dependencies. In practice, we find that more capable frontier-class LLMs tend to yield cleaner decompositions and more reliable graph construction.

\subsection{Sensitivity to SS-GED Hyperparameters}
\label{sec:ss_ged_hyperparameter_sensitivity}

To validate sensitivity of GraphEVAL with respect to $\beta$ and $\gamma$ hyperparameters (\Cref{sec:methodology}) , we vary $\beta$ between 0 and 1.0 with a step size of 0.2 and $\gamma \in \{0.5, 1.0, 2.5, 5.0, 10.0, 20.0\}$. We conducted the analysis on GPQA, MedQA and StrategyQA datasets, sampling 50 questions from each dataset (seed 42). \Cref{tab:beta_sensitivity} reports $\beta$ sensitivity with $\gamma = 5$ fixed, while \Cref{tab:gamma_sensitivity} reports $\gamma$ sensitivity with $\beta = 0.4$ fixed. In both tables, each cell reports PCC / GSC accuracy.

\textbf{GRCS Correlation results:} when $\gamma=5.0$ (the value we used in the main paper) and varying $\beta \in \{0.0, 0.2, 0.4, 0.6, 0.8, 1.0\}$, the Pearson correlation between GRCS and faithfulness (PCC) is very consistent. When $\beta=0.4$ (the value we used in the main paper) and varying $\gamma \in \{0.5, 1.0, 2.5, 5.0, 10.0, 20.0\}$, correlations are similarly stable, with some statistical shifts only at extreme boundary values (e.g., $\gamma=20.0$) where the RBF kernel becomes excessively sharp.

\textbf{GSC Accuracy results:} when fixing $\gamma=5.0$ (the value we used in the main paper) and varying $\beta \in \{0.0, 0.2, 0.4, 0.6, 0.8, 1.0\}$, GSC accuracy slightly dropped at the extremes (i.e., $\beta=0.0$ or $\beta=1.0$). This observation confirms that as long as the pipeline uses a blend of both structural and semantic similarities, downstream decoding is highly stable. When fixing $\beta=0.4$ (the value we used in the main paper) and varying $\gamma \in \{0.5, 1.0, 2.5, 5.0, 10.0, 20.0\}$, GSC accuracy remains practically unchanged.

\input{tables/ss_gedsensitivity}

\input{tables/ss_ged_sensitivity2}

\subsection{Sensitivity Analysis of \texorpdfstring{$\alpha$}{alpha} in GSC Medoid Selection}\label{sec:alpha_sensitivity_appendix}

\input{tables/alpha_appendix}

We study the sensitivity of $\alpha$, the GSC to the trade-off parameter in GSC medoid selection ($\cf$, \Cref{sec:methodology,sec_gsc_detailed_appendix}). Recall that $\alpha$ balances structural graph centrality against
node-level consensus. We evaluate $\alpha \in \{0.0,\,0.2,\,0.5,\,0.7,\,0.8,\,1.0\}$ across three datasets (GPQA, MedQA, StrategyQA) and all three
models, reporting accuracy change relative to our default $\alpha = 0.8$. Table~\ref{table:alpha_cv_table_appendix} shows that accuracy is \emph{stable} across
$\alpha \in [0.2, 1.0]$, with differences of at most $\pm 2\%$ in most
configurations.
The degenerate case $\alpha = 0.0$ (pure node-consensus scoring, ignoring
graph centrality) introduces higher variance across datasets and models, reflecting the instability
of medoid selection when the structural criterion is completely removed. 

\subsection{Effectiveness of $\pname$ for Uncertainty Quantification - SRC \& KRC Correlations}\label{sec:krc_src_section_appendix}

\emph{To extend the analysis of \Cref{sec_rq1_all} beyond PCC
%Pearson's linear correlation
}, we also report rank-based results using Spearman Rank (SRC) and Kendall Rank (KRC) coefficients in \Cref{fig:krc_src_appendix}. These results confirm the same GRCS behavior analyzed in the main section. Across almost all datasets and models, GRCS is consistently negatively correlated with faithfulness (in 13 cases out of 15, $\sim$ 87\%). %The gap is often large. 
For LLaMA~3.1~8B, GRCS outperforms the baselines on GSM8K, StrategyQA, and MedQA, with attenuation appearing only on GPQA, the hardest setting. For Phi-4, GRCS strongly outperforms baselines on BoolQ ($\eg$ achieving a KRC of -0.27, when all baselines correlations are weakly negative or positive), and shows competitive results in all the other settings. As noted in \Cref{sec_rq1_all}, GRCS strength attenutes for DeepSeek R1. While it is still negatively correlated on GSM8K, BoolQ, and MedQA, it only definitively outperforms all baselines on StrategyQA. GPQA remains the hardest benchmark. For both LLaMA~3.1~8B and DeepSeek~R1, GRCS flips to a positive correlation ($>0$) in both KRC and SRC. Topo-UQ and CoTA yield weak or entirely positive signals as well. In this setting, dispersion and entropy are the only metrics exhibiting relatively strong negative correlations.
\bem{Overall, the rank-based correlation results reinforce the main conclusion (\Cref{sec_rq1_all}) that GRCS is a robust metric for flagging unfaithful reasoning.}

\input{pic/krc_src_appendix}

\subsection{Global Topological Mapping}\label{sec:sec_top_mapping}
%\emph{To evaluate whether highly optimized LLMs possess true reasoning heterogeneity or suffer from structural mode collapse}, we conducted an adversarial ablation study. For queries where Graph-SC successfully identified a valid Medoid, we prompted the models at $T=0$ to solve the problem while strictly forbidding the use of the original Medoid's logic. We evaluated the resulting alternative trajectories using three metrics: Alternative Accuracy, Alternative faithfulness (via early answering), and Medoid-Alternative Distance.A robust reasoning engine should exhibit high distance (indicating a genuinely novel logical path) while maintaining high faithfulness and accuracy. Conversely, a drop in faithfulness or accuracy indicates that the model's apparent reasoning capabilities are heavily overfit to a single, fragile topological path.
\begin{comment}
\emph{To visually quantify the models' propensity to reasoning heterogeneity before perturbation}, %before actually perturbing the models, 
we first map the natural topology of their reasoning spaces. As \Cref{fig:combined_reasoning_topology_appendix} shows, we analyze LLM performance on the StrategyQA and GPQA datasets by mapping each query across two dimensions: structural incoherence (Divergence) %, closely related to GRCS as discussed in \Cref{sec:methodology_pipeline}) 
and generation heterogeneity (Entropy)%. For every question, we take the $N=20$ CoTs generated for the previous results and compute Divergence and Entropy over this set, yielding a single point that summarizes the structure and variability of the model’s reasoning.
, computed over the $N=20$ reasoning paths used in prior experiments.
%To characterize both the discrete topology and the underlying distribution of reasoning behaviors, we visualize this space using two complementary views: a scatter plot of individual queries and kernel density estimates (KDEs) defined over the same $(\text{Divergence},\text{Entropy})$ axes, which reveal the global density landscape of reasoning regimes.
Scatter plots capture query-level behavior, while Kernel Density Estimations (KDEs) reveal the global density landscape.
We then divide the 2D space into four quadrants, using the average $(\text{Divergence}, \text{Entropy})$ of our baseline model, LLaMA-3.1, as origin ($\mu_{div, ref}=0.31$, $\mu_{ent, ref}=0.85$). This allows us to  quantify four distinct reasoning regimes: \emph{Confident} ($\text{Divergence} < \mu_{div, ref}$, $\text{Entropy} < \mu_{ent, ref}$) indicates stable and structurally coherent reasoning across generations. \emph{Multi-Path} ($\text{Divergence} < \mu_{div, ref}$, $\text{Entropy} \ge \mu_{ent, ref}$) denotes a regime where reasoning remains coherent, yet the model successfully explores multiple alternative, valid reasoning trajectories. \emph{Noisy} ($\text{Divergence} \ge \mu_{div, ref}$, $\text{Entropy} < \mu_{ent, ref}$) suggests consistently incoherent or structurally fractured reasoning patterns that lack diversity. Finally, \emph{Confused} ($\text{Divergence} \ge \mu_{div, ref}$, $\text{Entropy} \ge \mu_{ent, ref}$) reflects both severe structural incoherence and chaotic variability in the generated reasoning chains.
DeepSeek R1 occupies a broad, %high-entropy convex hull that spans across both 
%broad 
high-entropy region spanning both the \emph{Multi-Path} and \emph{Confused} quadrants (with a mean of $\mu=(0.33, 1.03)$). This behavior is further supported by its KDE landscape, which portrays a wide, diffuse density region rather than a single dominant attractor. This means that, when uncertain, it explores many diverse reasoning paths. While some remain structurally coherent, others can be highly divergent. 
In contrast, %smaller models such as 
LLaMA~3.1~8B and Phi-4 %exhibit a more evident \emph{mode collapse}: their generations are more concentrated in low-entropy regions, and their KDE plots reveal sharp, singular attractor basins 
concentrate in lower-entropy regions with sharper KDE attractors, consistent with more rigid reasoning dynamics and stronger mode collapse. This concentration suggests comparatively rigid reasoning dynamics with limited exploration of alternative reasoning paths. 
\end{comment}
\emph{To visually quantify the models' propensity for reasoning heterogeneity before perturbation}, we map the natural topology of their reasoning spaces. As \Cref{fig:combined_reasoning_topology_appendix} shows, we analyze StrategyQA and GPQA by plotting the GLLMs' elicited CoTs for each question $q$ in a two-dimensional space defined by structural incoherence (Divergence) and generation heterogeneity (Entropy). For each question, we compute these quantities over the same $N=20$ CoTs used in prior experiments, yielding a single point that summarizes the structure and variability of the model’s reasoning. Scatter plots capture query-level behavior, while Kernel Density Estimations (KDEs) reveal the global density landscape.
We divide this space into four regimes using the baseline LLaMA-3.1 mean as the reference origin. \emph{Confident} corresponds to low Divergence and low Entropy, indicating stable and structurally coherent reasoning. \emph{Multi-Path} combines low Divergence with high Entropy, reflecting coherent exploration of multiple reasoning trajectories. \emph{Noisy} denotes high Divergence but low Entropy, suggesting consistently fractured reasoning with little diversity. \emph{Confused} captures simultaneously high Divergence and high Entropy, indicating both structural inconsistency and broad variability.
On StrategyQA, DeepSeek R1 occupies the broadest high-entropy region, spanning both the \emph{Multi-Path} and \emph{Confused} quadrants (mean $\mu=(0.33, 1.03)$), and its KDE forms a wide, diffuse basin rather than a single attractor. This suggests that, when uncertain, it explores a larger reasoning manifold: some paths remain mutually coherent, while others drift substantially. Phi-4 lies between the two extremes, while LLaMA~3.1~8B remains concentrated in lower-entropy regions with sharper density peaks, consistent with more rigid reasoning dynamics and stronger mode collapse.
GPQA preserves this same qualitative ordering, but under an overall compression of the entropy axis. This happens because this tasks is expert reasoning harder and more constraining than open domain reasoning. All three models shift downward, yet their relative structure remains stable: DeepSeek R1 still sustains the widest spread and continues to populate the \emph{Multi-Path} and \emph{Confused} regions, Phi-4 again acts as an intermediate regime, and LLaMA~3.1~8B collapses even more strongly toward the low-variance \emph{Confident} quadrant.
\bem{This analysis %tells that LLMs exhibit distinct reasoning regimes depending on scale, 
reveal distinct reasoning regimes across scales: from a more rigid mode collapse in smaller models to broad multi-path exploration in more capable ones. %By showing this natural capabilities, we establish the necessary foundation to adversarially ablate these primary reasoning paths and test whether they are genuinely load-bearing.
This topological difference motivates the necessity to adversarially ablate these primary reasoning paths and test whether they are genuinely essential.}
\input{pic/rq3_1_pics}

\subsection{Decoding Evaluation and Hybrid Audit at the Path Level}\label{sec:decoding_res_path_appendix}


\emph{To assess reasoning fidelity at the path level and characterize the nature of unfaithful reasoning within each decoding rule}, we extend the decoding audit of \Cref{sec:decoding_res}. %by transitioning from final-answer evaluation to a granular analysis of individual CoTs, 
While our main paper audit classified an SC answer as robust if the paths supporting its majority vote were predominantly faithful, here we execute a more granular analysis by evaluating each individual CoT \emph{independently}.
We distinguish between \textit{faithful} paths (where every inferential step follows logically from its antecedents) and \textit{unfaithful} paths (which reach the correct answer through a demonstrably flawed mechanism).  \Cref{fig:gsc_sc_verification_rate_apppedix} reports the percentage of paths within SC and GSC winning clusters that are faithful versus unfaithful, for the same models and datasets used in the main paper.  These results validate the question-level analysis performed in \Cref{sec:decoding_res}. For LLaMA 3.1 8B, unfaithful paths constitute a substantial fraction of SC winning clusters on harder benchmarks. On GPQA, 87\% of SC consensus paths are faithful, yet the remaining 13\% are unfaithful, while GSC retains 92\% faithful paths with only 8\% unfaithful. On MedQA, 50\% of SC paths are unfaithful, versus 0\% selected by GSC. On GSM8K, both methods perform comparably well, with SC at 90\% and GSC at 92\% faithful paths. For Phi-4, path-level fidelity is generally higher across all benchmarks, mirroring the question-level trend. Here, \bem{GSC achieves a higher path faithfulness across all complex benchmarks} (89\% vs 86\% on StrategyQA, 100\% vs 84\% on MedQA, 45\% vs 42\% on GPQA). For DeepSeek R1-Distill 70B, the path-level picture is the sharpest. In this case, \bem{GSC path level faithfulness is always $> 70\%$ across all benchmarks}, while SC never goes beyond 44\% ($p < 0.05$, Wilcoxon signed-rank test \cite{wilcoxon1945}).
\input{pic/path_level_appendix}

\subsection{Broad Population-Level Medoid Ablation - Additional Results
%\dpal{NOT READ}
}\label{sec:broad_abl_appendix_stratqa}

\emph{To extend the broad medoid ablation attacks performed in \Cref{sec:sec_rq3_broad_ablation} across diverse reasoning domains}, we repeat the same population-level protocol on GSM8K, MedQA, BoolQ, and GPQA (\Cref{fig:broad_ablation_fig_appendix}). 
The results on MedQA and GSM8K closely mirror the dynamic observed in the main paper. On GSM8K, both Llama 3.1 8B ($r=-0.18$, $p=0.010$) and Phi-4 ($r=-0.17$, $p=0.015$) exhibit significant negative linear correlations. On MedQA, Phi-4 shows a highly significant trend ($r=-0.38$, $p<0.001$), with Llama 3.1 8B exhibiting a marginally significant negative slope ($r=-0.17$, $p=0.088$). This confirms that in rigid deductive tasks and complex clinical reasoning, accuracy gains under ablation ($\Delta$Accuracy $> 0$) are coupled with drops in reasoning faithfulness ($\Delta$Faithfulness $< 0$), empirically capturing the ``lucky guess'' phenomenon. DeepSeek R1, consistent with its broader reasoning topology (\cf \Cref{sec:sec_top_mapping}) and our findings in \Cref{sec:sec_rq3_broad_ablation}, remains decoupled across both datasets ($\eg$, $r=-0.01$, $p=0.856$ on GSM8K). 
However, the linear relationship between $\Delta$Accuracy and $\Delta$Faithfulness attenuates on BoolQ and GPQA. On BoolQ, only Llama 3.1 8B shows a significant negative slope ($r=-0.14$, $p=0.041$), while Phi-4 and DeepSeek R1 show very weak or no significant linear association. On GPQA, no models exhibit significant correlations. As shown in our main results in \Cref{sec_rq2_all}, initial GSC accuracy on GPQA is extremely low ($\eg$, 19.3\% for Llama 3.1 8B). With so few initially correct reasoning paths to ablate, the potential for accuracy degradation ($\Delta$Accuracy $< 0$) is strictly constrained, resulting in noisy variance rather than linear degradation.
Crucially, across all domains, a dense cluster of points distributes along the $\Delta$Accuracy $= 0$ axis while extending deeply into negative $\Delta$Faithfulness. This dynamic is strongly quantified in MedQA. While ablation preserves accuracy in the vast majority of cases (77.0\% for Llama 3.1 8B, 94.0\% for Phi-4, and 95.7\% for DeepSeek R1), a significant portion of these exact points suffers a simultaneous drop in faithfulness (34.0\%, 24.0\%, and 16.1\% of all evaluated points, respectively).
\bem{These results strengthen our primary findings: across 3 of the 5 evaluated benchmarks, ablating the GSC medoid induces a significant negative correlation between accuracy and faithfulness for smaller GLLMs. Crucially, across all datasets and GLLM scales, the faithfulness degradation at $\Delta$Accuracy $= 0$ suggests that the medoid acts as a load-bearing path.}

\input{pic/broad_attack_appendix}
%\input{pic/broad_attack}

\subsection{%RQ3: Adversarial Vulnerability Analysis:
Targeted Adversarial Medoid Ablation
}\label{sec_target_appendix}

%\subsubsection{Targeted Adversarial Medoid Ablation}\label{sec:rq3_narrow}

%\emph{To determine whether the reasoning coherence measured by our framework reflects true topological heterogeneity or simply an artifact of mode collapse}, we conducted an adversarial ablation study. For each LLM, we isolated the marginal subset of queries where GSC derived the ground-truth answer (100\% accuracy) and won over standard SC, and prompted the models to re-evaluate each query while strictly forbidding the use of the logic contained within their original Medoid CoT. Because this ablation study strictly targets the marginal cases where standard majority voting fails and GSC uniquely succeeds, the sample sizes ($N$) are inherently small, representing the most difficult reasoning edge-cases in the datasets.
\input{tables/ablation_table}
\emph{To test whether the medoid identified by GSC is functionally important}, we perform an adversarial ablation on the small %narrow 
subset of questions where \bem{only} GSC is correct and SC is not. %For each such question, we prompt the model to answer again while explicitly forbidding the logic of the original medoid chain. 
%Because this probe targets only the marginal cases where GSC uniquely succeeds, the sample sizes are necessarily small. 
Therefore, this experiment is %intended as 
a stress test, complementary to the population-level ablation of \Cref{sec:sec_rq3_broad_ablation}.
Following \Cref{sec:methodology}, we evaluate the resulting alternative $N = 20$ CoTs across four dimensions: \textit{Ablated Accuracy} (AA), \textit{Ablated Faithfulness} (AF) (via Early-Answering truncation), \textit{Original Faithfulness} (OF) of the initial medoid, and \textit{Medoid Distance} (MD, normalized sequence dissimilarity). Because this subset is  defined by GSC's only wins, the original accuracy is $1.00$ across all configurations. Table~\ref{table:target_abl_table_results_appendix} summarizes our findings across (dataset, GLLM) pairs.
These results highlights different behaviors. First, in all but one case ($\ie$ DeepSeek R1 on MedQA), the GLLMs' ability to reach the correct final answer drops substantially, when it's forced to deviate from the GSC-selected medoid. Across BoolQ, GPQA, and StratQA, AA falls to between $0.333$ and $0.559$ for all GLLMs. Second, high MDs confirm that the accuracy drop does not happen because GLLMs fails to follow the attack prompt. Across almost all datasets, MDs range from $0.576$ to $0.995$. This suggests that, under adversarial conditions, all GLLMs are able to generate CoTs that are diverse from the ablated medoid. DeepSeek R1 consistently produces the highest MD (peaking at $0.995$ on MedQA and $0.935$ on StratQA), indicating it explores the most heterogenous paths when restricted (this validates our findings in \Cref{sec:sec_top_mapping} from an adversarial point of view). Third, in contrast to the almost uniform collapse in accuracy, the relationship between AF and OF depends on the GLLM and the domain. In general, AF exhibits high volatility. For instance, Llama 3.1 8B on StratQA drops from an OF of $0.657$ to an AF of $0.364$, while DeepSeek R1 on BoolQ rises from $0.274$ to $0.705$. This volatility is a direct consequence of the targeted nature of this subset. As noted in \Cref{sec:sec_rq3_broad_ablation}, faithfulness drops are strongly coupled with instances where models gain or preserve nominal accuracy (the "lucky guess" phenomenon). %Although this phenomenon is statistically more significant in smaller GLLMs ($\cf$, \Cref{sec:sec_rq3_broad_ablation}), the behavior of DeepSeek R1 on MedQA is an example of this (AA remains at 1.0, but AF dramatically goes to 0.0).
Although this dynamic is statistically more significant in smaller GLLMs (\cf \Cref{sec:sec_rq3_broad_ablation}), in this experiment it is clearly captured by DeepSeek R1 on MedQA, where accuracy is entirely preserved (AA = 1.000) but there is a complete loss of faithfulness (AF = 0.000). However, because the ablation in this specific subset significantly lowers GLLM' accuracy, the resulting AF scores reflect fragmented, unsuccessful reasoning paths rather than the uniform downward trend seen when accuracy remains close to its original values.
%Due to the page limit, \Cref{fig:medoid_ablation_fig} shows the results for GPQA and StrategyQA, and Appendix \rreva{ref} shows the results for the other datasets.
%Across all GLLMs on StrategyQA, the prompt attack successfully forces the generation of novel CoTs (distances in $0.74-0.93$ range). However, it also degrades the GLLM's ability to arrive at the correct answer. DeepSeek R1 achieves the most divergent alternative path (Distance: 0.93), but its AA %alternative accuracy 
%drops drastically to 39\%. Phi-4 and Llama 3.1 8B show similar accuracy collapses, falling to 50\% and 51\%, respectively. AF %Faithfulness 
%usually improves in more capable models, but drops with Llama 3.1 8B, highlighting the structural fragility of its reasoning space when its primary deduction path is removed.
%GPQA results follow this trend. DeepSeek R1 experiences a simultaneous collapse in both AA %alternative accuracy 
%(50\%) and AF %alternative faithfulness 
%(dropping from 0.55 to 0.33) when forced away from its medoid. Phi-4 and Llama mirror %again 
%this downward trend in AA. %accuracy. 
%\bem{Ultimately, these adversarial results validate our GSC decoding strategy. The medoid identified by the reasoning graph is not a simple cluster center but rather is the load-bearing ``Golden Path'' of the generation pool. By anchoring selection to this medoid path, GSC preserves the most structurally reliable reasoning.} 
%\bem{These adversarial results suggest that the medoid selected by GSC is often a load-bearing ``Golden Path'': when its logic is removed, models generate novel alternatives that frequently lose accuracy, even in instances where their underlying reasoning faithfulness actually improves. This indicates that GSC improves decoding by preserving a structurally central and functionally important reasoning path}.
\bem{While population-level ablation primarily exposes faithfulness drops ($\cf$, \Cref{sec:sec_rq3_broad_ablation}), this targeted test shows severe accuracy degradation and high faithfulness variance, confirming the GSC medoid acts as a load-bearing path.}

\section{Case Studies
%\dpal{START HERE}
}\label{sec:cases_appendix}

\subsection{Overview - Where GSC Catches Hallucinations and SC Fails}
This appendix details concrete cases where GSC successfully identifies correct answers supported by faithful reasoning paths, while standard SC selects answers produced by hallucinating or logically flawed reasoning chains. These cases illustrate three critical failure modes of majority voting: (1) \bem{shallow consensus on unfaithful reasoning}, (2) \bem{conflation of logical validity with numerical agreement}, and (3) \bem{fragmented answer space exploited by low-quality paths}.

\subsection{Case Study 1: The Hallucination Detection Case (Question: StrategyQA, bdaf032b5e375aeb9bfa)}
%"Would an Evander Holyfield 2020 boxing return set age record?.\nFor the final answer after your reasoning, answer either 'true' or 'false'"
This question is extrapolated from the StrategyQA common %d 
reasoning benchmark and its ID is bdaf032b5e375aeb9bfa. As \Cref{lst:1} shows, it asks if Bobby Jindal's high school mascot would eat kibble. The correct answer is \emph{true}: Bobby Jindal attended Baton Rouge Magnet High School, whose mascot is the \emph{Bulldog}, and a bulldog is a dog, which would eat kibble.
\begin{lstlisting}[
  style=promptstyle,
  caption={StrategyQA, Question ID bdaf032b5e375aeb9bfa},
  label={lst:1},
  emph={CRITICAL,CONSTRAINT,STRICTLY,FORBIDDEN,COMPLETELY,ALTERNATIVE,Guidelines,depends_on,Do,not,Question,final,answer,reasoning,alternative},
  escapeinside={(*@}{@*)}
]
"Would Bobby Jindal's high school mascot eat kibble?"
For the final answer after your reasoning, answer either 'true' or 'false'
(*@{\bfseries\color{blue} GOLD VALUE: true}@*)
\end{lstlisting}
We analyze and study the reasoning paths elicited using DeepSeek R1 as GLLM.
In this example, the $N=20$ CoTs produce 12 final \emph{false} answers and 8 final \emph{true} answers, so SC majority voting selects \emph{false}. GSC, however, selects \emph{true}, identifying a reasoning path that is more semantically and structurally coherent. SC fails because it blindly selects the most frequent answer, but that majority is not supported by a consistent underlying rationale. Instead, the \emph{false} CoTs are highly fragmented, as they converge on the same final label through mutually inconsistent hallucinated intermediate facts, including different schools and different mascots. As \Cref{tab:no_cot_fragmentation_jindall} shows, across the \emph{false} cluster, the model assigns different schools and different mascots, including \emph{Panthers}, \emph{Tigers}, \emph{Wildcats}, \emph{Alligators}, \emph{Eagles}, and \emph{Saints}. Thus, these traces agree only on the final label, while diverging sharply in the crucial, causal facts used to justify it. Their apparent consensus is therefore \bem{accidental} and \bem{unfaithful} rather than evidence of a stable underlying rationale.
By contrast, the \emph{true} cluster exhibits a highly consistent reasoning pattern. These traces repeatedly follow the same chain: \emph{Baton Rouge High} $\rightarrow$ \emph{Bulldogs} $\rightarrow$ \emph{dogs eat kibble}  $\rightarrow$ \bem{true}. In graph terms, they induce nearly identical reasoning structures, with high overlap in both nodes and edges. This makes the \emph{true} cluster internally coherent, even though it is numerically smaller than the \emph{false} cluster.
\input{tables/jidall}
To make the basis of medoid selection explicit, recall that GSC identifies the medoid by maximizing the GSC Score:
\[
\arg\max_{G_i}\left[\alpha \frac{C(G_i)}{\max_j C(G_j)}+(1-\alpha)P(G_i)\right],
\]
\Cref{lst:1_winner} shows the \bem{medoid CoT selected by GSC}, and provides a clear illustration of why GSC succeeds in this case. Unlike the hallucinated \emph{false} traces, this reasoning path is not only locally valid, but also \bem{collectively supported} by the broader sample of \emph{true} CoTs. It follows the correct causal chain -- \emph{Baton Rouge High School} $\rightarrow$ \emph{Bulldog} $\rightarrow$ \emph{dog} $\rightarrow$ \emph{kibble} $\rightarrow$ \bem{true} -- and this same semantic and structural pattern is repeatedly recovered across the \emph{true} cluster. Quantitatively, the selected medoid (CoT 01) achieves a total graph similarity of 12.4739, a path consensus of 0.5877, and the highest GSC score of 0.9527. As \Cref{fig:gsc_scores_jindall_fig_appendix} shows, other faithful \emph{true} traces receive similarly high scores, including CoT 08 (0.9519), CoT 07 (0.9470), CoT 10 (0.9440), and CoT 17 (0.9339), confirming that the correct answer is supported by a dense and internally consistent neighborhood of reasoning paths. 
\Cref{lst:1b} shows a case of a \bem{confident hallucination} (CoT 09), in which the reasoning chain is locally coherent but globally false. Each step follows plausibly from the previous one, yet the entire argument is anchored in the hallucinated intermediate facts (the wrong mascot). As a result, the trace appears structurally valid while still producing an incorrect final answer. GSC rejects this trace because its reasoning coherence is \bem{only local, not collective}: although CoT 09 is internally smooth, it is not supported by a stable cluster of semantically aligned causal reasomning facts. The surrounding \emph{false} traces reach the same answer through incompatible mascots and schools, yielding low pairwise similarity of the crucial, causal facts and a weak medoid. In fact, the hallucinated CoT 09 attains a substantially lower path consensus of 0.3421 and a lower combined score of 0.7795, reflecting that its apparent coherence is only local and is not shared by the broader \emph{false} cluster. In other words, GSC wins here not because it prefers a minority answer per se, but because it identifies that the minority answer is supported by the most internally coherent and reproducible reasoning structure in the sample. In contrast, the faithful \emph{true} traces repeatedly share the same core graph, so GSC promotes that cluster and suppresses this hallucinated one.
\bem{This case highlights the core advantage of GSC over standard SC. Majority voting is misled by coincidental agreement among diverse hallucinations, whereas GSC exploits structural and semantic similarity across reasoning traces. As a result, it discounts the fragmented \emph{false} cluster and instead selects the medoid of the coherent \emph{true} cluster, recovering the correct answer.}
\begin{lstlisting}[
  style=promptstyle,
  caption={StrategyQA, Question ID bdaf032b5e375aeb9bfa, \textbf{CoT 01 (Medoid CoT)}},
  label={lst:1_winner},
  emph={CRITICAL,CONSTRAINT,STRICTLY,FORBIDDEN,COMPLETELY,ALTERNATIVE,Guidelines,depends_on,Do,not,Question,final,answer,reasoning,alternative},
  escapeinside={(*@}{@*)}
]
0. Bobby Jindal attended Baton Rouge High School. [depends_on: none]
1. The mascot of Baton Rouge High School is the Bulldog. [depends_on: 0]
2. Bulldogs are dogs. [depends_on: 1]
3. Dogs typically eat kibble. [depends_on: 2]
4. Therefore, Bobby Jindal's high school mascot would eat kibble. [depends_on: 3]

(*@{\bfseries\color{blue} The final answer is: true}@*)
\end{lstlisting}

\begin{lstlisting}[
  style=promptstyle,
  caption={StrategyQA, Question ID bdaf032b5e375aeb9bfa, \textbf{CoT 09}},
  label={lst:1b},
  emph={CRITICAL,CONSTRAINT,STRICTLY,FORBIDDEN,COMPLETELY,ALTERNATIVE,Guidelines,depends_on,Do,not,Question,final,answer,reasoning,alternative},
  escapeinside={(*@}{@*)}
]
0. Bobby Jindal attended Baton Rouge Magnet High School. [depends_on: none]
1. The mascot of Baton Rouge Magnet High School is the Panthers. [depends_on: 0]
2. Panthers are wild big cats and do not eat kibble. [depends_on: 1]
3. Therefore, Bobby Jindal's high school mascot would not eat kibble. [depends_on: 2]

(*@{\bfseries\color{blue} The final answer is: false}@*)
\end{lstlisting}
\input{pic/gsc_scores_jindall}

\subsection{Case Study 2: The Assumption Fragmentation Case (Question: StrategyQA, a19804759885b694c56a)}
%"Would an Evander Holyfield 2020 boxing return set age record?.\nFor the final answer after your reasoning, answer either 'true' or 'false'"
This question is, again, extrapolated from the StrategyQA and its ID is a19804759885b694c56a. As \Cref{lst:2} shows, it asks whether one hundred thousand lolcat images could fit on a first-generation iPhone. The correct answer is \emph{true}: the first-generation iPhone was available in a 16GB version, and if each lolcat image is roughly 100KB, then 100{,}000 such images would require about 10GB of storage, which fits within that capacity.
\begin{lstlisting}[
  style=promptstyle,
  caption={StrategyQA, Question ID a19804759885b694c56a},
  label={lst:2},
  emph={CRITICAL,CONSTRAINT,STRICTLY,FORBIDDEN,COMPLETELY,ALTERNATIVE,Guidelines,depends_on,Do,not,Question,final,answer,reasoning,alternative},
  escapeinside={(*@}{@*)}
]
"Could a hundred thousand lolcats fit on a first generation iPhone?"
For the final answer after your reasoning, answer either 'true' or 'false'
(*@{\bfseries\color{blue} GOLD VALUE: true}@*)
\end{lstlisting}
We analyze and study the reasoning paths elicited using DeepSeek R1 as GLLM.
Also in this case, SC selects the most frequent answer, \emph{false}, that leads with 14 votes. On the other hand, GSC selected medoid CoT has \emph{true} as its final answer.
In this example, the core failure mode is not a single fabricated fact, but \bem{assumption fragmentation}. The incorrect traces do not agree on one stable rationale. Instead, they vary across at least two hidden assumptions: the storage capacity of the first-generation iPhone and the average size of each lolcat image. Some \emph{false} CoTs assume an 8GB model and conclude that $100{,}000 \times 100\text{KB} \approx 10\text{GB}$ cannot fit; others inflate the image size to 200KB, 300KB, or 500KB, making the total storage requirement much larger still (CoT 02, detailed in \Cref{lst:2b}, is an example). 
\begin{lstlisting}[
  style=promptstyle,
  caption={StrategyQA, Question ID a19804759885b694c56a, \textbf{CoT 02}},
  label={lst:2b},
  emph={CRITICAL,CONSTRAINT,STRICTLY,FORBIDDEN,COMPLETELY,ALTERNATIVE,Guidelines,depends_on,Do,not,Question,final,answer,reasoning,alternative},
  escapeinside={(*@}{@*)}
]
0. The first-generation iPhone has a maximum storage capacity of 8 gigabytes. [depends_on: none]
1. A typical lolcat image is approximately 100-500 kilobytes in size. [depends_on: none]
2. Converting the iPhone's storage to megabytes gives 8192 megabytes (8 GB = 8192 MB). [depends_on: 0]
3. Assuming an average lolcat size of 300 kilobytes (0.3 MB), the iPhone could store about 27306 images (8192 MB / 0.3 MB per image). [depends_on: 1,2]
4. 100,000 lolcats would require significantly more storage space than the iPhone's capacity. [depends_on: 3]
5. Therefore, a hundred thousand lolcats cannot fit on a first-generation iPhone. [depends_on: 4]

(*@{\bfseries\color{blue} The final answer is: false}@*)
\end{lstlisting}
By contrast, the faithful \emph{true} traces repeatedly instantiate the same core graph:
\emph{16GB model exists} $\rightarrow$ \emph{100KB per image} $\rightarrow$ \emph{100{,}000} $\times$ \emph{100KB} $\approx$ \emph{9.54 GB} $\rightarrow$ \emph{fits} $\rightarrow$ \bem{true}.
This pattern is exactly what's described in the GSC selected medoid CoT (CoT 05, \Cref{lst:2_winner}), and appears consistently in multiple CoTs, including CoTs 01, 06, 10, and 11, which all recover essentially the same quantitative reasoning chain. Although the wording varies slightly across traces, the semantic content and causal structure remain highly aligned. \Cref{fig:gsc_scores_iphone_fig_appendix} makes the selection mechanism visually explicit: the top of the ranking is populated primarily by coherent reasoning traces, with the GSC medoid (CoT 05) emerging from this dense neighborhood, whereas incoherent or hallucinated traces are more fragmented and tend to receive lower scores.
\begin{lstlisting}[
  style=promptstyle,
  caption={StrategyQA, Question ID a19804759885b694c56a, \textbf{CoT 05 (Medoid CoT)}},
  label={lst:2_winner},
  emph={CRITICAL,CONSTRAINT,STRICTLY,FORBIDDEN,COMPLETELY,ALTERNATIVE,Guidelines,depends_on,Do,not,Question,final,answer,reasoning,alternative},
  escapeinside={(*@}{@*)}
]
0. The first-generation iPhone had storage capacities of 4GB, 8GB, and 16GB. [depends_on: none]
1. Assuming each lolcat image is approximately 100KB, 100,000 lolcats would require about 10GB of storage. [depends_on: 0]
2. A 16GB iPhone could store 10GB of lolcats, leaving 6GB free. [depends_on: 1]
3. Therefore, 100,000 lolcats could fit on a 16GB first-generation iPhone. [depends_on: 2]

(*@{\bfseries\color{blue} The final answer is: true}@*)
\end{lstlisting}

\input{pic/gsc_scores_iphone}

\subsection{Case Study 3: Misordered Clinical Reasoning (Question: MedQA, 440)}
This question is extrapolated from MedQA and asks for the most appropriate \emph{initial} therapy for a 12-year-old boy with uncomplicated epistaxis (\Cref{lst:3}). The correct answer is \emph{D}: squeezing the nostrils manually for 10 minutes with the head elevated. This is the standard first-line management for stable anterior epistaxis before escalation to topical vasoconstrictors, packing, or other interventions \cite{msd_nosebleeds}. 

\vspace{2cm}
\begin{lstlisting}[
  style=promptstyle,
  caption={MedQA, Question ID a19804759885b694c56a},
  label={lst:3},
  emph={CRITICAL,CONSTRAINT,STRICTLY,FORBIDDEN,COMPLETELY,ALTERNATIVE,Guidelines,depends_on,Do,not,Question,final,answer,reasoning,alternative},
  escapeinside={(*@}{@*)}
]
"A 12-year-old boy is brought to the emergency department for the evaluation of persistent bleeding from his nose over the past hour. The bleeding started spontaneously. He has no history of a similar episode. He takes no medications. There is no history of abnormal bleeding in the family. His vital signs are within normal limits. On examination, he is pressing a gauze against his left nostril while hyperextending his head. The gauze is stained with blood and upon withdrawal of the gauze blood slowly drips out of his left nostrils. There is no bleeding from the right nostril. The remainder of the physical examination shows no abnormalities. Which of the following is the most appropriate initial therapy? 
Here are the answer options:
A) Anterior packing and topical antibiotics
B) Oxymetazoline nasal spray
C) Placement of an epinephrine gauze in the left nostril
D) Squeezing the nostrils manually for 10 minutes with the head elevated
Answer by selecting just one of the options."
(*@{\bfseries\color{blue} GOLD VALUE: D) Squeezing the nostrils manually for 10 minutes with the head elevated}@*)
\end{lstlisting}
We analyze the reasoning paths elicited using Phi-4 as GLLM. Here, the dominant failure mode is mainly related to \bem{misordered clinical reasoning}. Many incorrect CoTs prematurely escalate to invasive therapy, especially epinephrine gauze (option C. ), by assuming that first-line conservative management has already failed or by incorrectly reclassifying the bleed as more severe than the vignette supports. In particular, several traces treat the patient’s use of gauze as evidence that proper manual compression has already been attempted and was ineffective, even though the vignette does not state that bilateral compression for 10 minutes with head elevation has been performed. Other traces incorrectly infer posterior epistaxis from persistence alone and justify escalation on that basis. 
\Cref{lst:3b} illustrates this failure mode clearly. CoT 8 incorrectly interprets the presence of gauze as evidence that proper first-line manual compression has already failed, and therefore prematurely escalates to epinephrine gauze. The trace is locally coherent, but it is anchored in a false procedural assumption about what has already been tried. 
\begin{lstlisting}[
  style=promptstyle,
  caption={MedQA, Question ID 404, \textbf{CoT 08}},
  label={lst:3b},
  emph={CRITICAL,CONSTRAINT,STRICTLY,FORBIDDEN,COMPLETELY,ALTERNATIVE,Guidelines,depends_on,Do,not,Question,final,answer,reasoning,alternative},
  escapeinside={(*@}{@*)}
]
0. The boy is experiencing persistent nasal bleeding despite applying pressure, indicating the bleeding may be more severe than simple epistaxis. [depends_on: none]
1. Oxymetazoline nasal spray (Option B) is a vasopressor that can constrict blood vessels and is often used as a first-line treatment for mild epistaxis, but given the persistence and severity of this case, it may not be sufficient. [depends_on: 0]
2. Squeezing the nostrils (Option D) is a basic first-aid measure for epistaxis, but since the bleeding persists despite pressure, this method has already been attempted and is insufficient. [depends_on: 0]
3. Anterior packing and topical antibiotics (Option A) are used for severe or persistent epistaxis that does not respond to initial measures, but antibiotics are not necessary without signs of infection. [depends_on: 1, 2]
4. Placement of an epinephrine gauze (Option C) is appropriate as an initial therapy for severe epistaxis because epinephrine causes vasoconstriction, which can help control persistent bleeding. [depends_on: 0, 1, 2]
5. Given the severity and persistence of the bleeding, and the fact that initial basic measures have failed, epinephrine gauze is the most appropriate initial therapy. [depends_on: 4]


(*@{\bfseries\color{blue} The final answer is: C) Placement of an epinephrine gauze in the left nostril}@*)
\end{lstlisting}
The medoid CoT is (detailed in \Cref{lst:3_winner}) is correct because it preserves the correct treatment hierarchy: manual compression is first-line for uncomplicated anterior epistaxis, whereas oxymetazoline, epinephrine gauze, and packing are escalation steps. Although the trace contains some noisy supporting statements, it retains the key procedural ordering that defines the right answer.
\begin{lstlisting}[
  style=promptstyle,
  caption={MedQA, Question ID 404, \textbf{CoT 13 (Medoid CoT)}},
  label={lst:3_winner},
  emph={CRITICAL,CONSTRAINT,STRICTLY,FORBIDDEN,COMPLETELY,ALTERNATIVE,Guidelines,depends_on,Do,not,Question,final,answer,reasoning,alternative},
  escapeinside={(*@}{@*)}
]
0. The boy has a persistent nosebleed that has not stopped with initial measures like gauze packing, indicating a need for further intervention [depends_on: none].  
1. Anterior nosebleeds are a common issue in children and often respond well to initial conservative measures like nasal compression and topical vasoconstriction [depends_on: none].  
2. Oxymetazoline nasal spray can help by constricting blood vessels and is a non-invasive initial therapy for anterior nosebleeds [depends_on: 1].  
3. Squeezing the nostrils manually is a recommended first-line conservative treatment for anterior nosebleeds [depends_on: 1].  
4. Placement of an epinephrine gauze is typically used for more severe or recurrent nosebleeds when initial measures fail [depends_on: 3].  
5. Anterior packing is used for persistent bleeding that doesn't respond to initial conservative measures, and topical antibiotics can prevent infection from packing [depends_on: 4].  

(*@{\bfseries\color{blue} The final answer is: D) Squeezing the nostrils manually for 10 minutes with the head elevated.}@*)
\end{lstlisting}
\input{pic/gsc_scores_epistaxis}
Quantitatively, \Cref{fig:gsc_scores_epistaxis_fig_appendix} shows a particularly challenging regime: the medoid (CoT~13) is \emph{alone at the top} with the highest GSC score, while many of the immediately following traces are incorrect. Thus, GSC succeeds not because the correct cluster cleanly dominates the ranking, but because it isolates the single most central faithful path even when the surrounding reasoning pool is heavily contaminated by coherent but misordered clinical reasoning.

\section{Related Work}\label{sec:rel_work_appendix}
The purpose of this section is to provide a more comprehensive review of the literature discussed in \Cref{sec_rel_work}. 

\subsection{UQ Approaches}
We can divide existing Uncertainty Quantification (UQ) approaches for Large-Language Models into two primary categories, \emph{architecture-dependent} and \emph{architecture-agnostic}. Architecture-dependent approaches require direct access to the internal mechanisms of the model to estimate confidence ($\ie$, they rely on token-level probabilities, raw logits, hidden states, or activation patterns). They can involve training auxiliary classifiers on these internal representations or fine-tuning the LLM itself to explicitly output confidence scores alongside its predictions. On the other hand, Architecture-agnostic approaches treat the LLM as a closed system, and estimate uncertainty relying solely on the final generated outputs. Common techniques include sampling multiple responses or prompting the LLM to self-evaluate its own responses. 
Within the architecture-depedent category, \cite{kadavath2022language} train an additional internal ``value head'' to predict $P(IK)$, which represents the probability that the model actually ``knows'' the correct answer. Specifically, they define "knowing" not as an abstract concept, but as the empirical likelihood that the model will independently generate the correct response when taking multiple open-ended samples at unit temperature. This approach inherently requires probing specific token positions and internal logits to calculate confidence. Within architectures-asgnostic category, \cite{tian2023justask} extract well-calibrated confidence scores from RLHF-trained LLMs by prompting models to directly verbalize their confidence as text or numerical probabilities. They demonstrate that these verbalized confidences—especially when aggregated over multiple sampled answers—are significantly better-calibrated than the models' raw conditional probabilities.
Beyond direct prompting, several architecture-agnostic methods estimate uncertainty from the semantic consistency of sampled outputs. \cite{KuhnGalFarquhar2023} introduced \emph{Semantic Entropy}, which measures uncertainty by grouping generations that express the same underlying answer. Building on this idea, \cite{Farquhar2024SemanticEntropy} showed that semantic clustering is effective for hallucination detection. Similarly, \cite{LinTrivediSun2024} used semantic similarity graphs and their Laplacian spectra to identify unreliable outputs. However, these methods operate only at the level of the final answer and discard the intermediate reasoning structure.

More recent work has begun to incorporate structure. Topo-UQ \cite{da2025understanding}, for example, maps CoTs into topological graphs and uses structural dispersion as a proxy for uncertainty. Related inference frameworks such as \emph{Tree of Thoughts} \cite{Yao2023TreeOfThoughts} and graph-based reasoning \cite{BestaEtAl2024} further show that non-linear structures can represent richer dependencies than linear chains. Yet these methods are primarily designed to guide generation, not to quantify uncertainty across independently sampled CoTs post hoc.

A key limitation of purely topological approaches is that structural dispersion alone can miss important failure modes. In particular, it may fail under mode collapse, where models repeatedly produce structurally similar but flawed reasoning patterns \cite{ding2024breakchain}. This leaves a clear gap: uncertainty should account for both semantic validity and structural organization across the full reasoning manifold, motivating our $\pname$ framework.

\subsection{Sequence-Level Decoding and Structural Reasoning}
Decoding strategies dictate how an LLM navigates the vast distribution of possible reasoning paths to generate a final answer. The standard approach is \emph{greedy decoding}, which deterministically selects the highest-probability token at each step \cite{wei2022chainofthought}. While computationally efficient, greedy decoding is highly susceptible to cascading errors during complex tasks; a single hallucinated or incorrect token early in a Chain-of-Thought (CoT) trajectory locks the model into a suboptimal logical path, almost guaranteeing an incorrect final answer.
To mitigate the brittleness of single-path greedy decoding, \cite{wang2023selfconsistency} introduced \emph{Self-Consistency} (SC). Instead of relying on a single deterministic trajectory, SC samples a diverse set of reasoning paths using a non-zero temperature and selects the final answer via majority voting. By marginalizing over the intermediate reasoning steps, SC leverages the intuition that complex reasoning problems often have multiple valid logical pathways leading to the same correct conclusion, significantly improving accuracy over standard greedy decoding.
However, a critical limitation of Self-Consistency is that it aggregates consensus solely at the level of the final output. Because it inherently discards the logical structure and validity of the intermediate CoTs, SC is highly vulnerable to unfaithful reasoning---instances where flawed, collapsed, or contradictory logic accidentally converges on the majority-voted answer. While advanced inference frameworks like \emph{Tree of Thoughts} \cite{Yao2023TreeOfThoughts} and \emph{Graph of Thoughts} \cite{BestaEtAl2024} address structural reasoning by searching over branches during generation, they do not resolve the decoding problem. This gap highlights the need for a decoding mechanism that selects answers based on the structural and semantic consensus of the entire reasoning graph, rather than just the final token.
