# Supplementary material for: GRAPHEVAL: Quantifying Reasoning Uncertainty to Assess Trustworthiness in LLMs
Source: arXiv:2607.08017 source file (2026-12-02)
Supplement: Supplementary file 5 [file alpha_appendix.tex]

\begin{table}[H]
\centering
%\resizebox{\linewidth}{!}{%
\begin{tabular}{llr rrrrr}
\toprule
\multirow{2}{*}{\textbf{Dataset}}
  & \multirow{2}{*}{\textbf{Model}}
  & \textbf{GSC}
  & \multicolumn{5}{c}{$\Delta$ accuracy (pp) vs.\ $\alpha{=}0.8$} \\
\cmidrule(lr){4-8}
  &   & \textbf{@\,$\alpha{=}0.8$}
      & $\alpha{=}0.0$ & $\alpha{=}0.2$ & $\alpha{=}0.5$
      & $\alpha{=}0.7$ & $\alpha{=}1.0$ \\
\midrule
% ── StrategyQA ────────────────────────────────────────────────────────────
\multirow{3}{*}{StratQA}
  & Llama 3.1 8B  & 71.6 & $+2.2$           & $\phantom{+}0.0$ & $\phantom{+}0.0$ & $\phantom{+}0.0$ & $\phantom{+}0.0$ \\
  & Phi-4         & 76.7 & $-4.6$           & $\phantom{+}0.0$ & $\phantom{+}0.0$ & $\phantom{+}0.0$ & $\phantom{+}0.0$ \\
  & DeepSeek R1   & 78.2 & $-1.8$           & $-1.3$           & $+0.8$           & $+0.8$           & $+0.8$           \\
\midrule
% ── MedQA ─────────────────────────────────────────────────────────────────
\multirow{3}{*}{MedQA}
  & Llama 3.1 8B  & 52.0 & $+10.0$          & $\phantom{+}0.0$ & $\phantom{+}0.0$ & $\phantom{+}0.0$ & $\phantom{+}0.0$ \\
  & Phi-4         & 79.0 & $-3.0$           & $-2.0$           & $\phantom{+}0.0$ & $\phantom{+}0.0$ & $-2.0$           \\
  & DeepSeek R1   & 91.9 & $-1.0$           & $-2.0$           & $-1.0$           & $\phantom{+}0.0$ & $-1.0$           \\
\midrule
% ── GPQA ──────────────────────────────────────────────────────────────────
\multirow{3}{*}{GPQA}
  & Llama 3.1 8B  & 19.3 & $-1.0$           & $\phantom{+}0.0$ & $\phantom{+}0.0$ & $\phantom{+}0.0$ & $\phantom{+}0.0$ \\
  & Phi-4         & 32.8 & $+3.6$           & $\phantom{+}0.0$ & $\phantom{+}0.0$ & $\phantom{+}0.0$ & $\phantom{+}0.0$ \\
  & DeepSeek R1   & 52.4 & $\phantom{+}0.0$ & $\phantom{+}0.0$ & $-2.1$           & $+0.5$           & $\phantom{+}0.0$ \\
\bottomrule
\end{tabular}%
%}
\caption{
\label{table:alpha_cv_table_appendix}
    \textbf{Sensitivity of Graph-SC medoid selection to the trade-off parameter $\alpha$}.
    Each cell reports $\Delta$ accuracy (pp) relative to $\alpha{=}0.8$ (our default).
    Accuracy is stable across $\alpha \in [0.2, 1.0]$, with differences of at most
    $\pm 2$\,pp in most settings. $\alpha = 0.0$ shows substantially higher empirical variance
across configurations, reflecting the instability of medoid selection when the
primary structural criterion is removed.
}
\end{table}
